# Supplementary material for: Evolution of social behaviors in noisy environments
Source: arXiv:2510.05521 source file (2025-10-07)
Supplement: Supplementary file 1 [file SI.pdf]

# *Supplementary Information*
# Evolution of social behaviors in noisy environments

Guocheng Wang[1,2], Qi Su[3,4,5], Long Wang[1,6], Joshua B. Plotkin[2,7]

[1]Center for Systems and Control, College of Engineering, Peking University, Beijing 100871, China
[2]Department of Biology, University of Pennsylvania, Philadelphia, PA 19104, USA
[3]School of Automation and Intelligent Sensing, Shanghai Jiao Tong University, Shanghai 200240, China
[4]Key Laboratory of System Control and Information Processing, Ministry of Education of China, Shanghai 200240, China
[5]Shanghai Key Laboratory of Perception and Control in Industrial Network Systems, Shanghai 200240, China
[6]Center for Multi-Agent Research, Institute for Artificial Intelligence, Peking University, Beijing 100871, China
[7]Center for Mathematical Biology, University of Pennsylvania, Philadelphia, PA 19014, USA

## Contents

**1 Model description** **2**

**2 Derivation details** **3**
- 2.1 Two-strategy games . . . 3
  - 2.1.1 System equation . . . 3
  - 2.1.2 Evolutionary dynamics . . . 5
- 2.2 Multiple-strategy games . . . 7
  - 2.2.1 Rock-paper-scissors games . . . 9
  - 2.2.2 Other multi-strategy games . . . 13

**3 Model extensions** **14**
- 3.1 General fitness functions and update rules . . . 14
- 3.2 General noise structures . . . 17
  - 3.2.1 Multiple noise sources . . . 17
  - 3.2.2 Colored noise . . . 18
- 3.3 Small populations: fixation probability . . . 21

**Supplementary Figures** **37**

## 1 Model description

For a population of $N$ individuals, each individual can choose one of the two strategies called, generically, cooperation (C) or defection (D) for pairwise $2 \times 2$ games. Traditionally, the payoff structure, which can be viewed as the environment of the social interaction, is assumed to be deterministic and invariant. Here, we assume that the environment is subject to external fluctuations. Specifically, the payoff structure is supposed to have the following form

$$A = \bar{A} + \xi \Sigma = \begin{bmatrix} a & b \\ c & d \end{bmatrix} + \xi \begin{bmatrix} \tilde{a} & \tilde{b} \\ \tilde{c} & \tilde{d} \end{bmatrix}, \tag{1}$$

where $\bar{A}$ is the deterministic component of the payoff structure. $\xi$ is an unbiased random variable with unit variance ($\mathbb{E}(\xi) = 0$ and $\mathrm{Var}(\xi) = 1$), which reflects the environmental fluctuations.

Given there are $n_C$ cooperators in the population, the payoff of the two types of players are

$$\Pi_C(n_C, \xi) = \frac{(n_C - 1)(a + \xi\tilde{a}) + (N - n_C)(b + \xi\tilde{b})}{N - 1}, \tag{2a}$$

$$\Pi_D(n_C, \xi) = \frac{n_C(c + \xi\tilde{c}) + (N - n_C - 1)(d + \xi\tilde{d})}{N - 1}. \tag{2b}$$

These payoffs are transformed into fitness by the function. $f = \exp(s\Pi)$. Here $s$ is called the selection intensity, which measures to what degree the payoffs affect the evolutionary dynamics of types. In each generation (time step), the noise $\xi$ will be sampled (producing outcome $k$, say), and then all individuals play games and derive payoffs under the payoff matrix $A = \bar{A} + k\Sigma$.

We assume individuals update their strategies through the classic birth-death process. In each time step, an individual, denoted by $i$, is selected randomly with a probability proportional to its fitness to serve as a role model. And another player $j$ is selected randomly among the rest. Then, player $i$ copies $j$'s strategy. In a given time step, assume that the environmental fluctuation $\xi$ equals $k$. So the conditional probability that the number of cooperators increases or decreases by 1 in this time step is

$$T^+(n_C|\xi = k) = \frac{N - n_C}{N - 1} \frac{n_C f_C(n_C, k)}{n_C f_C(n_C, k) + (N - n_C) f_D(n_C, k)}, \tag{3a}$$

$$T^-(n_C|\xi = k) = \frac{n_C}{N - 1} \frac{(N - n_C) f_D(n_C, k)}{n_C f_C(n_C, k) + (N - n_C) f_D(n_C, k)}. \tag{3b}$$

Here, $f_C(n_C, k) = \exp(s\Pi_C(n_C, k))$ ($f_D(n_C, k) = \exp(s\Pi_D(n_C, k))$) is the fitness of cooperators (defectors) when there are $n_C$ cooperators in the population and $\xi = k$. Assume that the probability density function of $\xi$ is $p(k)$. Since the value of $\xi$ is randomly sampled in each time step, using the total probability theorem, we can compute the unconditional probability that the number of cooperators increases or decreases by one in each time step (regardless of the value of $\xi$). The unconditional probability is

$$T^+(n_C) = \mathbb{E}[T^+(n_C|\xi)] = \int T^+(n_C|\xi = k) p(k) \mathrm{d}k, \tag{4a}$$

$$T^-(n_C) = \mathbb{E}[T^-(n_C|\xi)] = \int T^-(n_C|\xi = k) p(k) \mathrm{d}k, \tag{4b}$$

Note that the system is a discrete Markov process, whose dynamics are exactly described by the transition probabilities $T^+(n_C)$ and $T^-(n_C)$.

# 2 Derivation details

## 2.1 Two-strategy games

### 2.1.1 System equation

We first derive the master equation of the stochastic system. We use $P(n_C, \tau)$ to denote the probability that at time step $\tau$, there are $n_C$ cooperators among the population. Then, the master equation is

$$\begin{aligned} P(n_C, \tau+1) - P(n_C, \tau) = T^+(n_C - 1)P(n_C - 1, \tau) + T^-(n_C + 1)P(n_C + 1, \tau) \\ - T^+(n_C)P(n_C, \tau) - T^-(n_C)P(n_C, \tau). \end{aligned} \tag{5}$$

By introducing the notation $x = n_C/N$ and $t = \tau/N$, and the probability density $\rho(x,t) = NP(n_C, \tau)$, we have

$$\begin{aligned} \rho(x, t+N^{-1}) - \rho(x,t) = T^+(x - N^{-1})\rho(x - N^{-1}, t) + T^-(x + N^{-1})\rho(x + N^{-1}, t) \\ - T^+(x)\rho(x,t) - T^-(x)\rho(x,t). \end{aligned} \tag{6}$$

We can expand the probability density and transition rates in Taylor series. Neglecting terms to higher order than $N^{-2}$, we get

$$\frac{\partial}{\partial t}\rho(x,t) = -\frac{\partial}{\partial x}[a(x)\rho(x,t)] + \frac{1}{2}\frac{\partial^2}{\partial x^2}\left[b^2(x)\rho(x,t)\right], \tag{7}$$

where $a(x) = T^+(x) - T^-(x)$ and $b(x) = \sqrt{[T^+(x) + T^-(x)]/N}$. This equation is the Fokker-Planck equation. Its corresponding Langevin equation is

$$\mathrm{d}x = [T^+(x) - T^-(x)]\mathrm{d}t + \sqrt{[T^+(x) + T^-(x)]/N}\,\mathrm{d}W_t, \tag{8}$$

where $W_t$ is a standard Wiener process. This approximation assumes the population size is large ($N \to \infty$), such that we can use a continuous variable $x$ to denote the state of the system ($n_C$) and the discrete Markov process can be approximated by continuous dynamics. Although the derivation above specifies the precise conditions required to make this approximation, in practice we also find this is a fairly accurate approximation even for relatively small populations (see Section 3.3 in Supplementary Note 3 and Supplementary Fig. 1).

In the subsequent derivation, we will show that $T^+ - T^-$ has the order of $s$. For a sufficiently large population ($\sqrt{1/N} \ll s$), the diffusion term $b(x)$ is sufficiently smaller than the deterministic term, which thus can be omitted. This also means the demographic noise can be ignored, which enables us to pinpoint the effects of environmental noise alone. For small populations, the diffusion term (demographic noise) cannot be ignored. The population will eventually become fixed (all individuals become cooperators or defectors). In this case, we study the fixation probability of the two types. The fixation probability for cooperators (defectors) is the probability that a single mutant cooperator (defector) can invade and replace the whole population otherwise full of defectors (cooperators). In this case, fixation is affected by the combined effects of deterministic payoffs, environmental noise, and demographic stochasticity (see section 3.3 in Supplementary Note 3). However, studying fixation probability alone masks the complex and intriguing dynamical patterns in the interior of state space, such as coexistence

in snowdrift game and oscillations in the rock-paper-scissors game. Thus, we focus primarily on the large-population limit, neglecting the diffusion term to obtain an ordinary differential equation

$$\dot{x} = T^+(x) - T^-(x). \tag{9}$$

We expand Eq. 3 in a Taylor series to derive a simple analytical approximation. Taking $T^+(n_C|\xi = k)$ as an example, it yields

$$\begin{aligned} T^+(n_C|\xi = k) =& \frac{N-n_C}{N-1} \frac{n_C f_C(n_C,k)}{n_C f_C(n_C,k) + (N-n_C) f_D(n_C,k)} \\ =& x(1-x)\frac{1}{x + (1-x)\frac{\exp[s(x(c+k\tilde{c})+(1-x)(d+k\tilde{d}))]}{\exp[s(x(a+k\tilde{a})+(1-x)(b+k\tilde{b}))]}}. \end{aligned} \tag{10}$$

For simplicity, we introduce the notation

$$\begin{aligned} \pi_C(x) = xa + (1-x)b, \quad \pi_D(x) = xc + (1-x)d, \\ \tilde{\pi}_C(x) = x\tilde{a} + (1-x)\tilde{b}, \quad \tilde{\pi}_D(x) = x\tilde{c} + (1-x)\tilde{d}. \end{aligned} \tag{11}$$

Here, $\pi_C$ and $\pi_D$ represent the deterministic payoff (also the expected payoff) of cooperators and defectors. $\tilde{\pi}_C$ and $\tilde{\pi}_D$ describe the intensity of fluctuations of cooperators' and defectors' payoffs.

For weak selection ($s \ll 1$), Eq. 10 can be expanded in a Taylor series, and we truncate it at order $s^2$, which yields

$$\begin{aligned} T^+(x|\xi = k) =& x(1-x)\frac{1}{x + (1-x)\exp[s(\pi_D - \pi_C + k(\tilde{\pi}_D - \tilde{\pi}_C))]} \\ =& x(1-x)\frac{1}{1 + (1-x)[s(\pi_D - \pi_C + k(\tilde{\pi}_D - \tilde{\pi}_C)) + \frac{s^2}{2}(\pi_D - \pi_C + k(\tilde{\pi}_D - \tilde{\pi}_C))^2]} \\ =& x(1-x)[1 - s(1-x)(\pi_D - \pi_C + k(\tilde{\pi}_D - \tilde{\pi}_C)) \\ &+ s^2(x^2 - \frac{3}{2}x + \frac{1}{2})(\pi_D - \pi_C + k(\tilde{\pi}_D - \tilde{\pi}_C))^2]. \end{aligned} \tag{12}$$

Similarly, for $T^-(x|\xi = k)$ we have

$$\begin{aligned} T^-(x|\xi = k) =& x(1-x)[1 - sx(\pi_C - \pi_D + k(\tilde{\pi}_C - \tilde{\pi}_D)) \\ &+ s^2(x^2 - \frac{1}{2}x)(\pi_C - \pi_D + k(\tilde{\pi}_C - \tilde{\pi}_D))^2]. \end{aligned} \tag{13}$$

Then, substituting Eq. 12 and 13 into Eq. 4, and remembering $\mathbb{E}(\xi) = 0$ and $\mathbb{E}(\xi^2) = 1$, we obtain

$$\begin{aligned} T^+(x) =& \mathbb{E}[T^+(x|\xi)] \\ =& x(1-x)[1 - s(1-x)(\pi_D - \pi_C) - s(1-x)(\tilde{\pi}_D - \tilde{\pi}_C)\mathbb{E}(\xi) \\ &+ s^2(x^2 - \frac{3}{2}x + \frac{1}{2})\left((\pi_D - \pi_C)^2 + 2(\pi_D - \pi_C)(\tilde{\pi}_D - \tilde{\pi}_C)\mathbb{E}(\xi) + (\tilde{\pi}_D - \tilde{\pi}_C)^2\mathbb{E}(\xi^2)\right)] \\ =& x(1-x)\left[1 - s(1-x)(\pi_D - \pi_C) + s^2(x^2 - \frac{3}{2}x + \frac{1}{2})\left((\pi_D - \pi_C)^2 + (\tilde{\pi}_D - \tilde{\pi}_C)^2\right)\right], \end{aligned} \tag{14a}$$

$$T^-(x) = x(1-x)\left[1 - sx(\pi_C - \pi_D) + s^2(x^2 - \frac{1}{2}x)\left((\pi_C - \pi_D)^2 + (\tilde{\pi}_C - \tilde{\pi}_D))^2\right)\right]. \tag{14b}$$

Thus we have

$$T^+(x) - T^-(x) = x(1-x)\left[s(\pi_C - \pi_D) + s^2\left(\frac{1}{2} - x\right)((\pi_C - \pi_D)^2 + (\tilde{\pi}_C - \tilde{\pi}_D)^2)\right], \tag{15a}$$

$$T^+(x) + T^-(x) = 2x(1-x) + o(s). \tag{15b}$$

Here, the order of magnitude for $\tilde{\pi}_C$ and $\tilde{\pi}_D$ is crucial. We assume that the deterministic payoff $\pi_C$ and $\pi_D$ has order $O(1)$. If $\tilde{\pi}_C$ and $\tilde{\pi}_D$ is much smaller than $\sqrt{\frac{1}{s}}$ (i.e. $\sqrt{s}\tilde{\pi}_C \sim \sqrt{s}\tilde{\pi}_D \ll 1$ and $s(\tilde{\pi_C} - \tilde{\pi}_D)^2 \ll 1$), the term of $s^2$ in Eq. 15a can be ignored, and the dynamics simplifies to the classic replicator dynamics

$$\dot{x} = sx(1-x)(\pi_C - \pi_D). \tag{16}$$

This means very weak noise has little effect on the dynamics. If $\tilde{\pi}_C$ and $\tilde{\pi}_D$ are much larger than $\sqrt{\frac{1}{s}}$) (i.e. $\sqrt{s}\tilde{\pi}_C \sim \sqrt{s}\tilde{\pi}_D \gg 1$ and $s(\tilde{\sigma_C} - \tilde{\sigma}_D)^2 \gg 1$), the term of $s^2$ in Eq. 15a is dominant, and the dynamics of the system are totally determined by the noise. Then, the system equation Eq. 9 becomes

$$\dot{x} = s^2 x(1-x)\left(\frac{1}{2} - x\right)(\tilde{\pi}_C - \tilde{\pi}_D)^2. \tag{17}$$

This system has only one stable equilibrium $x = 1/2$. In this case, the population dynamics has a similar pattern with snowdrift games.

In this paper, we focus on the case of

$$\tilde{a} \sim \tilde{b} \sim \tilde{c} \sim \tilde{d} \sim \tilde{\pi}_C \sim \tilde{\pi}_D \sim s^{-\frac{1}{2}}, \tag{18}$$

which yields $s^2(\pi_C - \pi_D)^2 \sim O(s^2)$ and $s^2(\tilde{\pi}_C - \tilde{\pi}_D)^2 \sim O(s)$. In this regime the evolutionary outcome depends on the combination of two factors: deterministic payoffs and environmental fluctuations. For convenience, we rescale Eq. 1 by setting

$$\begin{bmatrix} \sigma_a & \sigma_b \\ \sigma_c & \sigma_d \end{bmatrix} = \sqrt{s}\begin{bmatrix} \tilde{a} & \tilde{b} \\ \tilde{c} & \tilde{d} \end{bmatrix}. \tag{19}$$

We omit the orders higher than $O(s)$ in Eq. 15a and then obtain

$$\dot{x} = sx(1-x)\left[\pi_C - \pi_D + \left(\frac{1}{2} - x\right)(\sigma_C - \sigma_D)^2\right]. \tag{20}$$

We find that if the environment is constant (i.e. $\sigma_a = \sigma_b = \sigma_c = \sigma_d = 0$) or $\sigma_C = \sigma_D$ (i.e., $\sigma_a = \sigma_c$ and $\sigma_b = \sigma_d$), this equation simplifies to the classic replicator equation, which means noise has no effects on the evolutionary outcome in these cases.

In the above derivation, we only make use of the expectation and variance of $\xi$ to derive the system equation. The specific distribution of $\xi$ is not used. Thus, this analysis remains consistent for a broad range of distributions, such as a normal distribution or Bernoulli distribution ($\mathbb{P}(\xi = -1) = \mathbb{P}(\xi = 1) = 0.5$).

### 2.1.2 Evolutionary dynamics

For sufficiently large populations, the evolution process is totally characterized by Eq. 20. Based on this equation, we can analyze the long-term outcomes and the stability of equilibrium points.

Since the noise matrix $\Sigma$ has four parameters, it is difficult to explore all cases of $\Sigma$. We focus on a special, but realistic, case in which payoffs of larger magnitude suffer larger fluctuations. For simplicity, we analyze the case when the noise intensity is proportional to the payoff, i.e.,

$$\begin{bmatrix} \sigma_a & \sigma_b \\ \sigma_c & \sigma_d \end{bmatrix} = k\begin{bmatrix} a & b \\ c & d \end{bmatrix}, \tag{21}$$

In this case, we define $E = a - c$ and $F = b - d$. The replicator equation Eq. 20 becomes

$$\dot{x} = sx(1-x)[F + (E-F)x]\left[k^2(F + (E-F)x)\left(\frac{1}{2} - x\right) + 1\right]. \tag{22}$$

This equation always has two equilibrium points on the boundaries $x = 0$ and $x = 1$. In what follows, we analyze only the equilibrium points in the interior, $(0,1)$. We discuss the dynamics for two scenarios:

**(I)** If $E - F = 0$ (i.e., $a - b - c + d = 0$), the equation becomes

$$\dot{x} = -sx(1-x)k^2F^2\left(x - \frac{1}{2} - \frac{1}{k^2F}\right). \tag{23}$$

If $\frac{1}{2} + \frac{1}{k^2F} \in (0,1)$, the system has a stable interior equilibrium point, which means the population dynamics is similar to a snowdrift game. If $\frac{1}{2} + \frac{1}{k^2F} \geq 1$, $\dot{x} > 0$ is always satisfied, and cooperation is the dominant strategy. If $\frac{1}{2} + \frac{1}{k^2F} \leq 0$, $\dot{x} < 0$ is always satisfied and defectors take over the population.

A typical example of this scenario is donation games. For donation games, the cooperator provides a benefit $\mathscr{B}$ to his opponent at a cost $\mathscr{C} > 0$, but the defector pays nothing. The deterministic payoff matrix $\bar{A}$ is

$$\begin{bmatrix} \mathscr{B} - \mathscr{C} & -\mathscr{C} \\ \mathscr{B} & 0 \end{bmatrix}. \tag{24}$$

Thus $F = -\mathscr{C}$. Apart from the equilibrium points $x = 0$ and $x = 1$, there are another equilibrium point

$$x_e = \frac{1}{2} - \frac{1}{k^2\mathscr{C}}. \tag{25}$$

Due to $\mathscr{C} > 0$, $x_e$ is always smaller than 1/2. If $k \leq \sqrt{2/\mathscr{C}}$, $x_e$ does not exist. Like the classic replicator dynamics, defection takes over the whole population. However, if $k > \sqrt{2/\mathscr{C}}$, $x_e$ is an interior stable equilibrium and $x = 0$ is no longer stable. The game dynamics is changed as if individuals are playing a snowdrift game where cooperators and defectors coexist in the long run.

**(II)** If $E - F \neq 0$, we have

$$\dot{x} = sk^2(E-F)^2x(1-x)(x-x^*)\left[(x-x^*)\left(\frac{1}{2} - x\right) + \frac{1}{k^2(E-F)}\right], \tag{26}$$

where

$$x^* = \frac{d-b}{a-b-c+d} \tag{27}$$

is the equilibrium point of the classic replicator equation. And we define

$$K = \frac{1}{k^2(E-F)} = \frac{1}{k^2(a-b-c+d)}. \tag{28}$$

Since $sk^2(E-F)^2$ is always positive and thus does not affect the dynamical patterns, the dynamics is totally determined by the two parameters $x^*$ and $K$. The sign of $K$ is the same as the sign of $E - F$ (i.e., $a - b - c + d$). For the classic replicator equation ($k = 0$), there are four cases:

(1) $\{x^* < 0$ and $E - F < 0\}$ or $\{x^* > 1$ and $E - F > 0\}$ (prisoner's dilemma): In this case, $\dot{x} < 0$ holds for all $x \in (0,1)$. Thus, defection is the dominant strategy.

(2) $\{x^* < 0$ and $E - F > 0\}$ or $\{x^* > 1$ and $E - F < 0\}$ (harmony game): In this case, $\dot{x} > 0$ holds for

all $x \in (0,1)$. Thus, cooperation is the dominant strategy.
(3) $0 < x^* < 1$ and $E - F > 0$ (coordination game): In this case, there is an interior unstable equilibrium point. And the two boundary points are stable ($x = 1$ and $x = 0$). All trajectories converge to full cooperation or full defection.
(4) $0 < x^* < 1$ and $E - F < 0$ (coexistence game): In this case, there is an interior stable equilibrium point. Starting from any initial states, the system will finally converge to this interior equilibrium.

However, if we consider the environmental noise, the right side of Eq. 26 is a quintic polynomial, which has at most five roots. Two roots ($x = 0$ and $x = 1$) are on the boundary. So we focus on the number of roots in the interior of $(0,1)$ of the function

$$f(x) = (x - x^*)^2 \left(\frac{1}{2} - x\right) + K(x - x^*). \tag{29}$$

By discussing how many roots of $f(x)$ are in $[0,1]$ and their stabilities, we can classify the dynamical patterns into seven cases. Here, we omit the specific computation details and only illustrate results in Figure 3 in the main text.
(i) For case (1) and case (2), we find that as $k$ varies, apart from the full defection (case (1)) or full cooperation (case (2)), the evolutionary outcome may also produce the coexistence of cooperation and defection if $E - F > 0$. If $E - F < 0$, the long-term outcomes can be either a single coexistence state, or a state with one stable interior equilibrium and one stable equilibrium on the boundary.
(ii) For case (3), as $k$ varies, the population dynamics can be transformed to have two interior stable equilibrium, or one interior stable equilibrium and one stable equilibrium on the boundary.
(iii) For case (4), as $k$ varies, the population dynamics can only be transformed into a pattern with two interior stable equilibria.

Evolutionary dynamics producing two interior stable equilibria, or one stable equilibrium in the interior and one on the boundary can never be seen in classic evolutionary dynamics of two strategy games without noise. These results show that environmental noise tends to break the stability of the states on the boundary and provide more stability in the interior.

Although we only focus on the case that the noise intensity is proportional to the deterministic payoff, for general noise intensity settings, there are still seven kinds of dynamical patterns as we mentioned above (also see Figure 3 in the main text). Specifically, for the general replicator equation Eq. 20, there are still at most three equilibrium points in the interior of $[0,1]$. For a quintic polynomial, there are at most eight kinds of dynamical patterns as shown in Tab. 1. However, the eighth dynamical pattern can never occur since the fifth-order term in the replicator equation Eq. 20 is

$$s(\sigma_a - \sigma_b - \sigma_c + \sigma_d)^2 x^5, \tag{30}$$

whose coefficient is always positive, which means the eighth pattern can never occur.

## 2.2 Multiple-strategy games

In this section, we consider games with multiple strategies, $m > 2$. The payoff structure is given by

$$\begin{pmatrix} a_{11} & \cdots & a_{1m} \\ \vdots & \ddots & \vdots \\ a_{m1} & \cdots & a_{mm} \end{pmatrix} + \frac{\xi}{\sqrt{s}} \begin{pmatrix} \sigma_{11} & \cdots & \sigma_{1m} \\ \vdots & \ddots & \vdots \\ \sigma_{m1} & \cdots & \sigma_{mm} \end{pmatrix}, \tag{31}$$

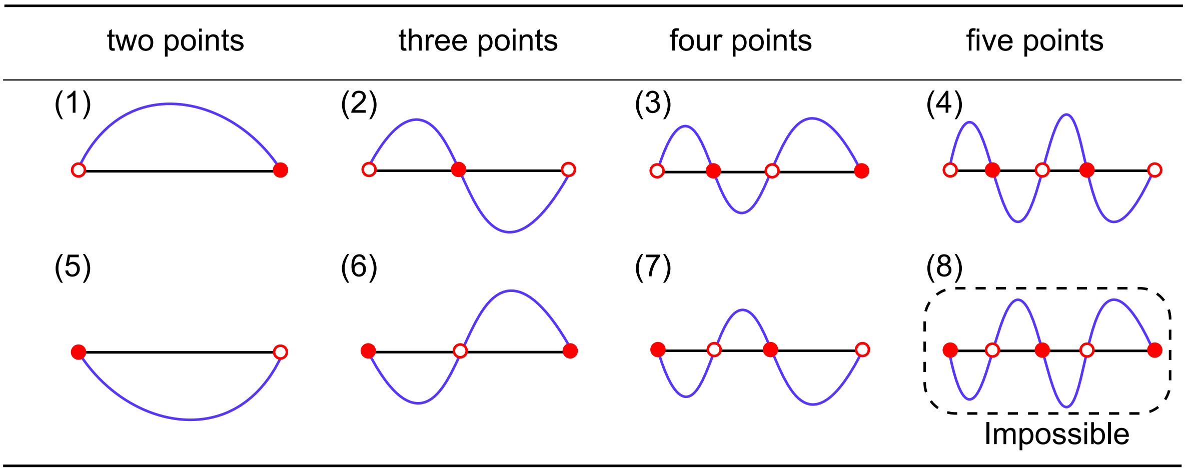


Supplementary Table 1: **Seven possible dynamical patterns.** For a quintic polynomial, it has at most five roots. Since the definition domain of the replicator equation is $[0,1]$, we only care about how many equilibrium points are in $[0,1]$. There are four scenarios: there are two, three, four, or five equilibrium points in $[0,1]$ ($x=0$ and $x=1$ always exist). For each scenario, there are two kinds of dynamical patterns which are determined by the direction that the polynomial goes through each point. For the eight cases, case (8) can never occur since the coefficient of the highest-order term of the polynomial is always positive.

which means a player adopting strategy $i$ receives payoff $a_{ij}+\xi\sigma_{ij}/\sqrt{s}$ when interacting with a player adopting strategy $j$. Suppose the number of individuals adopting strategy $i$ is $n_i$. The population composition can be expressed by an $m$-tuple $[x_1,\cdots,x_m]$, where $x_i$ is the frequency of strategy $i$ ($x_i = n_i/N$). We define the deterministic payoff and noise intensity for players adopting strategy $i$:

$$\pi_i = \sum_{j=1}^{m} a_{ij}x_j, \tag{32a}$$

$$\sigma_i = \sum_{j=1}^{m} \sigma_{ij}x_j. \tag{32b}$$

Under the birth-death updating rule, the probability that the number of $i$-players increases or decreases by one is

$$T_i^+ = \mathbb{E}\left[\frac{n_i \exp[s(\pi_i+\xi\sigma_i/\sqrt{s})]}{\sum_{j=1}^{m} n_j \exp[s(\pi_j+\xi\sigma_j/\sqrt{s})]}\frac{N-n_i}{N-1}\right] \approx \mathbb{E}\left[\frac{x_i \exp[s(\pi_i+\xi\sigma_i/\sqrt{s})]}{\sum_{j=1}^{m} x_j \exp[s(\pi_j+\xi\sigma_j/\sqrt{s})]}(1-x_i)\right], \tag{33a}$$

$$T_i^- = \mathbb{E}\left[\frac{\sum_{j\neq i} n_j \exp[s(\pi_j+\xi\sigma_j/\sqrt{s})]}{\sum_{j=1}^{m} n_j \exp[s(\pi_j+\xi\sigma_j/\sqrt{s})]}\frac{n_i}{N-1}\right] \approx \mathbb{E}\left[\frac{\sum_{j\neq i} x_j \exp[s(\pi_j+\xi\sigma_j/\sqrt{s})]}{\sum_{j=1}^{m} x_j \exp(\pi_j+\xi\sigma_j/\sqrt{s})}x_i\right]. \tag{33b}$$

Using similar techniques as 2.1.1, we can derive the modified replicator equations in the presence of noise. The equation for the frequency of strategy $i$ is given by

$$\dot{x}_i = sx_i\left[\pi_i - \bar{\pi} + \frac{1}{2}((\sigma_i-\bar{\sigma})^2 - \mathrm{Var}(\sigma))\right], \tag{34}$$

where

$$\bar{\pi} = \sum_j x_j \pi_j, \tag{35a}$$

$$\bar{\sigma} = \sum_j x_j \sigma_j, \tag{35b}$$

$$\mathrm{Var}(\sigma) = \sum_{j=1}^{m} x_j (\sigma_j - \bar{\sigma})^2. \tag{35c}$$

Here, $\bar{\pi}$ and $\bar{\sigma}$ describe the average payoff and average noise intensity in the population. The quantity $\mathrm{Var}(\sigma)$ represents the variance of noise intensity in the population. This equation shows that when all individuals have identical noise intensity (i.e., $\sigma_{1j} = \sigma_{2j} = \cdots = \sigma_{mj}$ for all $j$.), environmental fluctuation has no effect on the dynamics compared to the classic replicator equation.

For simplicity, we still focus on the case when noise intensity is proportional to the deterministic payoff matrix. That is

$$\sigma_{ij} = k a_{ij}. \tag{36}$$

Then, Eq. 34 becomes

$$\dot{x}_i = s x_i \left[ \pi_i - \bar{\pi} + \frac{k^2}{2} \left( (\pi_i - \bar{\pi})^2 - \mathrm{Var}(\pi) \right) \right], \tag{37}$$

where

$$\mathrm{Var}(\pi) = \sum_{j=1}^{m} x_j (\pi_j - \bar{\pi})^2. \tag{38}$$

### 2.2.1 Rock-paper-scissors games

To show how environmental noise affects evolutionary dynamics, we first consider a classic three-strategy game — rock-paper-scissors (RPS) game. The general RPS game has the following payoff matrix

$$\begin{pmatrix} 0 & -\alpha & \beta \\ \beta & 0 & -\alpha \\ -\alpha & \beta & 0 \end{pmatrix}. \tag{39}$$

For the RPS game, let $x, y, z$ denote the frequencies of the three strategies R, P, and S. Due to the relation of $x + y + z = 1$, this system is actually two-dimensional. We choose $x$ and $y$ to be the two independent variables, and the replicator equations are

$$\dot{x} = s x \left[ \pi_R - \bar{\pi} + \frac{k^2}{2} \left( (\pi_R - \bar{\pi})^2 - \mathrm{Var}(\pi) \right) \right], \tag{40a}$$

$$\dot{y} = s y \left[ \pi_P - \bar{\pi} + \frac{k^2}{2} \left( (\pi_P - \bar{\pi})^2 - \mathrm{Var}(\pi) \right) \right]. \tag{40b}$$

If $k = 0$, this simplifies to the classic replicator equation:

$$\dot{x} = s x (\pi_R - \bar{\pi}), \tag{41a}$$

$$\dot{y} = s y (\pi_P - \bar{\pi}). \tag{41b}$$

For these two systems (Eq. 40 and 41), they share an identical interior equilibrium point $x = y = z = 1/3$, denoted by $e^*$. In what follows, we investigate the stability of this fixed point.

We linearize Eq. 40 and 41 in the neighborhood of $e^*$. Their Jacobians at $e^*$ are the same, given by

$$\frac{s}{3}\begin{bmatrix} -\beta & -\alpha-\beta \\ (\alpha+\beta) & \alpha \end{bmatrix}. \tag{42}$$

Thus, the stability of $e^*$ does not depend on the intensity of noise ($k$) but is only determined by $\alpha$ and $\beta$. The two eigenvalues of $e^*$ are

$$\lambda_1 = \frac{s(\alpha-\beta)}{6} + i\frac{s\sqrt{3}}{6}(\alpha+\beta), \lambda_2 = \frac{s(\alpha-\beta)}{6} - i\frac{s\sqrt{3}}{6}(\alpha+\beta), \tag{43}$$

According to the sign of eigenvalues, we can classify the dynamics into three scenarios. If $\alpha > \beta$, $e^*$ is an unstable focus (spiral source). If $\alpha < \beta$, $e^*$ is a stable focus (spiral sink). If $\beta = \alpha$, $e^*$ is a center equilibrium (see Figure 4 in the main text).

Although these analyses of $e^*$ only predict the dynamics in the neighborhood of $e^*$, prior studies have already shown that the stability of $e^*$ determines the globe dynamics when $k = 0$ (no noise)[1, 2]. For Eq. 41, if $\alpha > \beta$, all trajectories converge to the boundary spirally, and all trajectories converge to $e^*$ spirally for $\alpha < \beta$. When $\alpha = \beta$, all trajectories are separate closed orbits. However, in what follows, we show that $k > 0$ (environmental noise) can induce a stable limit cycle. Before this, we first introduce a lemma.

**Lemma 2.1** (Andronov-Hopf bifurcation theorem [3])**.** Consider the 2-dimensional system

$$\dot{x} = f_\mu(x, y), \tag{44a}$$

$$\dot{y} = g_\mu(x, y), \tag{44b}$$

where $\mu$ is a parameter. Suppose it has an equilibrium point $e^* = (x^*, y^*)$. Denote the eigenvalues of its linearized system about the equilibrium point as $\lambda(\mu), \bar{\lambda}(\mu) = \mathrm{Re}_\mu(\lambda) \pm i\mathrm{Im}_\mu(\lambda)$. For $\mu = 0$, the real part of the eigenvalues vanishes and the imaginary part still exists (i.e. $\mathrm{Re}_0(\lambda) = 0, \mathrm{Im}_0(\lambda) = \omega \neq 0$). If the following nondegeneracy conditions hold:

**(AH.1)**

$$\frac{\mathrm{dRe}_\mu(\lambda)}{\mathrm{d}\mu}\Big|_{\mu=0} = d \neq 0. \tag{45}$$

**(AH.2)** $l_1(0) \neq 0$, where $l_1(\mu)$ is the first Lyapunov coefficient. $l_1(0)$ is given by

$$l_1(0) = \frac{1}{16}(f_{xxx} + f_{xyy} + g_{xxy} + g_{yyy}) + \frac{1}{16\omega}(f_{xy}(f_{xx} + f_{yy}) - g_{xy}(g_{xx} + g_{yy}) - f_{xx}g_{xx} + f_{yy}g_{yy}). \tag{46}$$

Here $f_{xy}$ represents $\partial^2 f/(\partial x \partial y)$ (other terms are similar). Then a unique curve of periodic solutions bifurcations from the $e^*$ for a close enough value $\mu > 0$ if $l_1(0)d < 0$ or a close enough value $\mu < 0$ if $l_1(0)d > 0$. $e^*$ is a stable fixed point for $\mu > 0$ (resp. $\mu < 0$) and an unstable fixed point for $\mu < 0$ (resp. $\mu > 0$) if $d < 0$ (resp. $d > 0$). The periodic solutions are stable (resp. unstable) if $e^*$ is unstable (resp. stable) on the side of $\mu = 0$ where the periodic solutions exist. The amplitude of the periodic orbits grows like $\sqrt{|\mu|}$ and the periods tend to $2\pi/|\omega|$. The bifurcation is called supercritical if the orbits are stable, and subcritical if they are unstable.

For convenience, in the RPS games, we define $\mu = \alpha - \beta$. From Eq. 43, we have

$$\mathrm{Re}_0(\lambda) = 0, \mathrm{Im}_0(\lambda) = \frac{s\sqrt{3}}{6}(\alpha + \beta), \tag{47a}$$

$$d = \frac{s}{6}, \tag{47b}$$

$$l_1(0) = -\frac{s}{2}\alpha^2 k^2. \tag{47c}$$

When $k \neq 0$, $l_1(0)$ is always negative. Thus, for $k \neq 0$, $l_1(0) < 0$ is always satisfied. According to Lemma. 2.1, we can find a limit cycle for $\mu > 0$ (i.e., $\alpha > \beta$). For $\mu > 0$, $e^*$ is unstable, thus the limit cycle is stable, which is a supercritical bifurcation. The amplitude of the limit cycle grows as $O(\sqrt{\alpha - \beta})$. Furthermore, by numerical computation, we find that the amplitude of the limit cycle is also influenced by the noise intensity $k$: as $k$ increases, the diameter of the limit cycle becomes smaller (see Figure 4 in the main text).

For $\beta = \alpha$ or $\beta > \alpha$, the interior point $e^*$ is stable. Although environmental noise cannot induce a limit cycle, numerical computation shows that it accelerates the evolution toward $e^*$.

In the main text, we show that in the regime of $\alpha > \beta$, for small $k$ (but non-zero), the limit cycle is globally stable, but for large $k$, the limit cycle is only locally stable. Here, we derive the analytical condition to predict when it is globally stable.

In the RPS games, we can prove that the evolutionary equation Eq. 40 has a unique interior equilibrium point, that is $e^*$.

**Lemma 2.2.** In the RPS games, for arbitrary $k$, the system Eq. 40 has only one interior equilibrium point $e^*$.

*Proof.* Given Eq. 40, the interior equilibrium points should satisfy the following equations:

$$\pi_R - \bar{\pi} + \frac{k^2}{2}\left[(\pi_R - \bar{\pi})^2 - \mathrm{Var}(\pi)\right] = 0, \tag{48a}$$

$$\pi_P - \bar{\pi} + \frac{k^2}{2}\left[(\pi_P - \bar{\pi})^2 - \mathrm{Var}(\pi)\right] = 0, \tag{48b}$$

$$\pi_S - \bar{\pi} + \frac{k^2}{2}\left[(\pi_S - \bar{\pi})^2 - \mathrm{Var}(\pi)\right] = 0, \tag{48c}$$

which implies

$$\pi_R - \bar{\pi} + \frac{k^2}{2}(\pi_R - \bar{\pi})^2 = \pi_P - \bar{\pi} + \frac{k^2}{2}(\pi_P - \bar{\pi})^2 = \pi_S - \bar{\pi} + \frac{k^2}{2}(\pi_S - \bar{\pi})^2. \tag{49}$$

This equation will be satisfied only when

$$\pi_R = \pi_P = \pi_S, \tag{50}$$

which solves the unique equilibrium point $e^*$. □

Since there is a unique interior equilibrium point, all other equilibrium points are on the boundary. Whether the limit cycle is globally stable depends on the stability of these equilibria on the boundary. If all these equilibria are unstable, the limit cycle is globally stable. Since the three strategies are symmetric, in order to calculate the equilibrium point on the boundary, we only need to study any two strategies. We choose strategies $R$ and $P$ to illustrate the analysis.

For a population only containing strategies $R$ and $P$, the game actually becomes a prisoner's dilemma (strategy $R$ is dominant). we use $x$ to denote the proportion of $R$, and thus the proportion of $P$ is $1-x$. Substituting $y = 1-x$ into Eq. 40, we can solve all equilibrium points. Apart from the two trivial points $x = 0$ and $x = 1$, there are three non-trivial equilibrium points:

$$x_1 = \frac{-3\alpha k^2 + \beta k^2 - k\sqrt{16\alpha - 16\beta + \alpha^2 k^2 + 2\alpha\beta k^2 + \beta^2 k^2}}{4k^2(\beta - \alpha)}, \tag{51a}$$

$$x_2 = \frac{-3\alpha k^2 + \beta k^2 + k\sqrt{16\alpha - 16\beta + \alpha^2 k^2 + 2\alpha\beta k^2 + \beta^2 k^2}}{4k^2(\beta - \alpha)}, \tag{51b}$$

$$x_3 = \frac{\alpha}{\alpha - \beta}. \tag{51c}$$

Since $\alpha > \beta$, we can verify that $x_1 > 1$ and $x_3 > 1$. The condition that $x_2$ lies in $(0,1)$ is $k^2\alpha > 2$. We can check that this condition is actually consistent with Figure 3 in the main text, which gives the condition when a prisoner's dilemma can be transformed into a coexistence game.

Thus, if $k^2\alpha < 2$, apart from the three homogeneous states $(1,0,0)$, $(0,1,0)$ and $(0,0,1)$, the unique equilibrium state is $e^* = (1/3, 1/3, 1/3)$. We have already shown that all three homogeneous states are unstable and $e^*$ is unstable. Thus, the limit cycle is globally stable.

If $k^2\alpha > 2$, there is only one equilibrium point on each boundary (the population consists only of two strategies). Thus, apart from the three homogeneous states and $e^*$, there are another three equilibrium points

$$e_1 = (x_2, 1-x_2, 0), \quad e_2 = (0, x_2, 1-x_2), \quad e_3 = (1-x_2, 0, x_2). \tag{52}$$

Due to the symmetry, the three points have identical stability. Thus, we only need to check the stability of one equilibrium (e.g., $e_3$). By computing the Jacobian of Eq. 40 at $e_3$, we have

$$\begin{bmatrix} J_{11} & * \\ 0 & J_{22} \end{bmatrix}. \tag{53}$$

Here, $J_{11}$ is always negative, as shown in Fig. 3 (the game between strategy $R$ and $P$ is a prisoner's dilemma in the upper-right region of Fig. 3, where the population dynamics has one stable equilibrium if $k^2\alpha > 2$) and Fig. 4 ($e_1$, $e_2$ and $e_3$ are always stable in the direction along the boundary since it is a coexistence game) in the main text. Thus, to investigate whether $e_1$ is stable, we need only check the stability in the direction perpendicular to the boundary (i.e., the sign of $J_{22}$). By some basic manipulations, we can compute that

$$\begin{aligned} J_{22}|_{e_3} = {} & (4\alpha^4 + 7\alpha\beta^3 + 14\alpha^2\beta^2 + 7\alpha^3\beta + 4\beta^4)k^2 + (24\alpha^2\beta - 24\alpha\beta^2 - 16\beta^3 + 16\alpha^3) \\ & -(5\alpha\beta^2 + 5\alpha^2\beta + 4\beta^3 + 4\alpha^3)k\sqrt{16(\alpha-\beta) + (\alpha+\beta)^2 k^2}. \end{aligned} \tag{54}$$

The condition for globally stable limit cycle is $J_{22} < 0$, i.e.,

$$0 < k < \frac{\sqrt{2}(\alpha + 2\beta)}{\sqrt{\alpha(\alpha^2 + \beta^2 + \alpha\beta)}}, \tag{55}$$

and otherwise, the limit cycle is locally stable.

If $\alpha \leq \beta$, there are no limit cycles, and the interior equilibrium $(1/3, 1/3, 1/3)$ is stable. However, more intense fluctuations (large $k$) can also make the interior equilibrium become only locally stable.

Small $k$ guarantees that it is globally stable. In this case, $x_3 < 0$ is always satisfied. According to Fig. 3 in the main text (bottom-left region), $x_1$ and $x_2$ may both exist. However, even if $x_1$ exists, it is unstable. Thus we only need to check the stability of $x_2$. The derivation is the same as the above case. Thus, the interior equilibrium $(1/3, 1/3, 1/3)$ is globally stable if Eq. 55 is satisfied.

#### 2.2.2 Other multi-strategy games

Apart from RPS games, we can also analyze other multi-strategy games. For three strategy games, we also investigated cases when one strategy is a dominant strategy or three strategies coexist. For these two kinds of games, environmental fluctuations can also produce more interior equilibria and enhance interior stability (see Supplementary Fig. 4).

We can likewise study games with four strategies, focusing on payoff structures where each strategy dominates another strategy circularly, similar to the property of RPS games. In such cases as well, environmental noise can yield stable periodic solutions and strengthen the coexistence of different phenotypes (see Supplementary Fig. 5).

# 3 Model extensions

## 3.1 General fitness functions and update rules

For a game with $m$ strategies. Based on the above discussion, the dynamics of the strategy $i$'s ratio $x_i$ is totally determined by the probability that the number of $i$-player increases or decreases by one (i.e. $T_i^+$ and $T_i^-$). Given the payoff structure and the fitness function $f_i = f(s\Pi_i)$, $T_i^+$ and $T_i^-$ are functions of all strategies' frequencies and the selection intensity $s$. Denote $\mathbf{x} = [x_1, x_2, \cdots, x_m]$ and $\Pi = [\Pi_1, \Pi_2, \cdots, \Pi_m]$. $T_i^+$ and $T_-^i$ can be expressed by $T_i^+(\mathbf{x}, s)$ and $T_i^-(\mathbf{x}, s)$.

Expanding $T_i^+$ and $T_i^-$ in a Taylor series of $s$, we have

$$T_i^+(\mathbf{x}, s) = T_i^+(\mathbf{x}, 0) + s\sum_{j=1}^{m} \frac{\partial T_i^+}{\partial s\Pi_j}\Big|_{\Pi=\mathbf{0}} \Pi_j + \frac{s^2}{2}\sum_{j,k} \frac{\partial^2 T_i^+}{\partial(s\Pi_j)\partial(s\Pi_k)}\Big|_{\Pi=\mathbf{0}} \Pi_j\Pi_k + o(s^2), \tag{56a}$$

$$T_i^-(\mathbf{x}, s) = T_i^-(\mathbf{x}, 0) + s\sum_{j=1}^{m} \frac{\partial T_i^-}{\partial s\Pi_j}\Big|_{\Pi=\mathbf{0}} \Pi_j + \frac{s^2}{2}\sum_{j,k} \frac{\partial^2 T_i^-}{\partial(s\Pi_j)\partial(s\Pi_k)}\Big|_{\Pi=\mathbf{0}} \Pi_j\Pi_k + o(s^2), \tag{56b}$$

where $T_i^+(\mathbf{x}, 0) = T_i^-(\mathbf{x}, 0)$. We denote

$$A_i^+(j) = \frac{\partial T_i^+}{\partial s\Pi_j}\Big|_{\Pi=\mathbf{0}}, \tag{57a}$$

$$A_i^-(j) = \frac{\partial T_i^-}{\partial s\Pi_j}\Big|_{\Pi=\mathbf{0}}, \tag{57b}$$

$$B_i^+(jk) = \frac{\partial^2 T_i^+}{\partial(s\Pi_j)\partial(s\Pi_k)}\Big|_{\Pi=\mathbf{0}}. \tag{57c}$$

$$B_i^-(jk) = \frac{\partial^2 T_i^-}{\partial(s\Pi_j)\partial(s\Pi_k)}\Big|_{\Pi=\mathbf{0}}. \tag{57d}$$

Given $\Pi_i = \pi_i + \sigma_i\xi/\sqrt{s}$, we can derive the system equation of evolution. For the deterministic case (i.e., $\sigma_i = 0$ holds for all $i$), we have

$$T_i^+(\mathbf{x}, s) = T_i^+(\mathbf{x}, 0) + s\sum_{j=1}^{m} A_i^+(j)\pi_j + \frac{s^2}{2}\sum_{j,k} B_i^+(jk)\pi_j\pi_k + o(s^2), \tag{58a}$$

$$T_i^-(\mathbf{x}, s) = T_i^-(\mathbf{x}, 0) + s\sum_{j=1}^{m} A_i^-(j)\pi_j + \frac{s^2}{2}\sum_{j,k} B_i^-(jk)\pi_j\pi_k + o(s^2). \tag{58b}$$

Omitting the terms with orders higher than $s$, the system equation is

$$\dot{x}_i = \mathbb{E}[T_i^+ - T_i^-] = s\left(\sum_{j=1}^{m} A_i^+(j)\pi_j - \sum_{j=1}^{m} A_i^-(j)\pi_j\right). \tag{59}$$

If the environment fluctuations exist, we have

$$T_i^+(\mathbf{x}, s) = T_i^+(\mathbf{x}, 0) + s\sum_{j=1}^{m} A_i^+(j)\pi_j + \frac{s}{2}\sum_{j,k} B_i^+(jk)\sigma_j\sigma_k\xi^2 + o(s), \tag{60a}$$

$$T_i^-(\mathbf{x}, s) = T_i^-(\mathbf{x}, 0) + s\sum_{j=1}^{m} A_i^-(j)\pi_j + \frac{s}{2}\sum_{j,k} B_i^-(jk)\sigma_j\sigma_k\xi^2 + o(s). \tag{60b}$$

Then, the system equation is

$$\dot{x}_i = \mathbb{E}[T_i^+ - T_i^-] = s\left(\sum_{j=1}^{m} [A_i^+(j) - A_i^-(j)]\pi_j\right) + \frac{s}{2}\left(\sum_{j,k} [B_i^+(jk) - B_i^-(jk)]\sigma_j\sigma_k\right). \tag{61}$$

Comparing Eq. 61 and Eq. 59, we can find that when

$$B_i^+(jk) \neq B_i^-(jk) \tag{62}$$

holds for an arbitrary $(i,j,k)$, the environmental fluctuation has influences on the evolutionary dynamics. Moreover, Eq. 62 is equivalent to

$$\frac{\partial^2 T_i^+}{\partial s^2}\bigg|_{s=0} = \frac{\partial^2 T_i^-}{s^2}\bigg|_{s=0}. \tag{63}$$

Apart from the birth-death process, there are some other classic updating rules, such as the death-birth process, imitation process, and pairwise comparison. We can verify that apart from pairwise comparison, environmental fluctuations also influence the population dynamics of the death-birth process and the imitation process. For the pairwise comparison, the probabilities that the number of $i_{\text{th}}$ strategy increases and decreases by one are

$$T_i^+ = x_i \sum_{j=1}^{m} \frac{x_j}{1+\exp(s(\Pi_j - \Pi_i))}, \tag{64a}$$

$$T_i^- = x_i \sum_{j=1}^{m} \frac{x_j}{1+\exp(s(\Pi_i - \Pi_j))}. \tag{64b}$$

(64c)

Then we have

$$\frac{\partial^2 T_i^+}{\partial s^2}\bigg|_{s=0} = \frac{\partial^2 T_i^-}{\partial s^2}\bigg|_{s=0} = 0. \tag{65a}$$

So environmental fluctuations have no effects on the population dynamics.

Furthermore, for the death-birth process and imitation process, given a fitness function, the system equation is the same as the birth-death process since the updating probabilities ($T^+$ and $T^-$) of these three processes are identical when the population size is large. So in the following, we can focus on the birth-death process and the results for death-birth and imitation processes are totally the same (see Supplementary Fig. 7).

For the birth-death process, we consider a general form of fitness function $f_i = f(s\Pi_i)$. Then, using similar methods, we can obtain the system equation:

$$\dot{x}_i = s x_i \left[\delta_1(M_1^2 - \sigma_i M_1) + \frac{\delta_2}{2}(\sigma_i^2 - M_2) + \pi_i - \bar{\pi}\right], \tag{66}$$

where

$$\delta_1 = \frac{f'(0)}{f(0)}, \quad \delta_2 = \frac{f''(0)}{f'(0)}, \tag{67}$$

and $\bar{\sigma}$ and $M_2$ is the first and second moment of $\sigma_i$, given by

$$\bar{\sigma} = \sum_{i=1}^{m} x_i \sigma_i, \tag{68a}$$

$$M_2 = \sum_{i=1}^{m} x_i \sigma_i^2. \tag{68b}$$

Here $\delta_1$ is always positive, which describes how fast fitness increases with payoffs. $\delta_2$ is positive if the fitness is convex and is negative if the fitness function is concave. If we regard the fitness function as

the utility function in terms of economics, $\delta_2$ describes the risk preference of the utility function and it equals $-ARA$, where $ARA$ is the Absolute Risk Aversion proposed by Pratt and Arrow [4, 5, 6]. $\delta_2 < 0$ describes risk aversion and $\delta_2 > 0$ describes risk seeking. Here risk aversion means a stochastic payoff yields lower expected fitness compared with a deterministic payoff (identical to the mean of the stochastic payoff), and risk-seeking means a stochastic payoff leads to higher expected fitness (Supplementary Fig. 6). For the classic fitness function $f_i = \exp(s\Pi_i)$ ($\delta_1 = \delta_2 = 1$), Eq. 66 simplifies to Eq. 34.

Note that for the classic exponential fitness ($\exp(s\Pi)$), the evolutionary dynamics has a nice property the same as the classic replicator dynamics that the evolutionary outcome only depends on the difference of fluctuating intensities of different types. So, if we assume the intensity of fluctuation is proportional to the baseline payoff, the dynamics only depends on the payoff difference of strategies. Adding identical payoffs on all individuals will not affect the dynamics. However, for general fitness, the evolutionary dynamics also depends on the specific values of all individuals' payoffs.

To show the generality of our results, here we study two other fitness functions which correspond to the case of $\delta_2 = 0$ and $\delta_2 < 0$.

**(A) $\delta_2 = 0$ (linear fitness)**

Here, $\delta_2 = 0$ implies $f''(0) = 0$. We choose a fitness function $f_i = 1 + s\pi_i$ to study the evolutionary dynamics. For this fitness function, the replicator equation becomes

$$\dot{x}_i = sx_i\left[\pi_i - \bar{\pi} + M_1(M_1 - \sigma_i)\right]. \tag{69}$$

By assuming $\sigma_i = k\pi_i$, we have

$$\dot{x}_i = sx_i(1 - k^2\bar{\pi})(\pi_i - \bar{\pi}). \tag{70}$$

Compared with the classic replicator equation, this equation also shows that the environment can yield extra interior equilibria that satisfy $k^2\bar{\pi} = 1$. We choose examples to show these results in Supplementary Fig. 8.

This means environmental noise can influence the population dynamics even for linear fitness functions. This effect arises from the non-linearity of the birth-death rule. We can consider a simple example to provide some intuitions. If there are two types cooperators and defectors in the population whose deterministic payoffs ($\pi_C$ and $\pi_D$) are both zero. Thus their real payoffs totally depend on the fluctuations (i.e., $\Pi_C = \sigma_C\xi$) and $\Pi_D = \sigma_D\xi$. In one generation, under the birth-death rule, the probabilities that the number of cooperators ($n_C$) increase by one or decrease by one are $x(1-x)\frac{1+s\sigma_C\xi}{1+s\bar{\sigma}\xi}$ and $x(1-x)\frac{1+s\sigma_D\xi}{1+s\bar{\sigma}\xi}$. Thus the expected increment of $n_C$ in each generation is

$$\mathbb{E}(n_C|\xi) = x(1-x)\frac{1+s\sigma_C\xi}{1+s\bar{\sigma}\xi} - x(1-x)\frac{1+s\sigma_D\xi}{1+s\bar{\sigma}\xi} = x(1-x)\frac{s(\sigma_C - \sigma_D)\xi}{1+s\bar{\sigma}\xi}. \tag{71}$$

For a symmetric fluctuation such as $\xi = \pm\epsilon$ with equal likelihood, the overall expected change of $n_C$ is

$$\mathbb{E}(n_C) = s^2x(1-x)\frac{(\sigma_C - \sigma_D)(-2\bar{\sigma}\epsilon^2)}{1-(s\bar{\sigma})^2}. \tag{72}$$

This implies that cooperators are expected to increase in number if $\sigma_C < \sigma_D$ and otherwise decrease. This effect stems from the non-linearity of the updating rule. We illustrate this in Supplementary Fig. 6.

**(B) $\delta_2 < 0$ (concave fitness)**

Here we choose a fitness function $f_i = 2 - \exp(-s\pi_i)$, where $\delta_1 = 1$ and $\delta_2 = -1$. For this fitness function, the replicator equation becomes

$$\dot{x}_i = sx_i \left[ \pi_i - \bar{\pi} + M_1(M_1 - \sigma_i) - \frac{1}{2}(\sigma_i^2 - M_2) \right]. \tag{73}$$

By assuming $\sigma_i = k\pi_i$, we have

$$\dot{x}_i = sx_i \left[ \pi_i - \bar{\pi} + k^2\bar{\pi}(\bar{\pi} - \pi_i) - \frac{k^2}{2}\left(\pi_i^2 - \overline{(\pi^2)}\right) \right]. \tag{74}$$

For two strategy games and three strategy games, we show that the environment can still produce more interior equilibria and limit cycles in RPS games (Supplementary Fig. 8).

These results verify that our results remain qualitatively consistent for different fitness functions and stress the strong influence of environmental fluctuations on evolutionary dynamics.

## 3.2 General noise structures

### 3.2.1 Multiple noise sources

In the above discussion, we focus on the case that the environmental noise is governed by a single noise source (random variable $\xi$), which also means the fluctuations in all elements of the payoff matrix are correlated. In this section, we explore the scenario that the payoff structure suffers fluctuations with multiple noise sources, which implies the fluctuations are controlled by multiple independent random variables.

Here, we still focus on the classic exponential fitness function ($\exp(s\Pi_i)$). For a game with $m$ strategies, the payoff matrix is given by $A$. Each elements $A_{ij}$ of $A$ is

$$A_{ij} = a_{ij} + \frac{1}{\sqrt{s}}\epsilon_{ij}, \tag{75}$$

where $\epsilon_{ij}$ is a Gaussian random variable. For an $m$-strategy game, the payoff matrix has $m^2$ elements. Then the covariance of $\epsilon_{ij}$ and $\epsilon_{hk}$ is

$$\mathrm{Cov}(\epsilon_{ij}, \epsilon_{hk}) = \sigma_{ij,hk}. \tag{76}$$

The covariance structure of noise is given by an $m^2 \times m^2$ matrix. In this case, the system equation can still be derived using a similar method. Denote the noise of strategy $i$'s payoff is $\epsilon_i$, which has the following expression

$$\epsilon_i = \sum_{j=1}^{m} \epsilon_{ij} x_j. \tag{77}$$

Then the system equation still has a similar form as Eq. 34:

$$\dot{x}_i = sx_i \left[ \pi_i - \bar{\pi} + \frac{1}{2}(\mathbb{E}((\epsilon_i - \bar{\epsilon})^2) - \mathrm{Var}(\epsilon)) \right], \tag{78}$$

where

$$\bar{\epsilon} = \sum_{j=1}^{m} x_j \epsilon_j = \sum_i \sum_j x_i \epsilon_{ij} x_j, \tag{79a}$$

$$\mathrm{Var}(\epsilon) = \sum_i x_i \mathbb{E}((\epsilon_i - \bar{\epsilon})^2). \tag{79b}$$

For the simple case that we considered in the main text (i.e., $\epsilon_{ij} = \sigma_{ij}\xi$), this equation simplifies to Eq. 34. For another special case, we assume that each element of the payoff matrix suffers independent noise (i.e., $\epsilon_{ij} = \sigma_{ij}\xi_{ij}$ where $\xi_{ij}$ is a standard Gaussian variable), which means the payoff matrix is given by

$$\begin{pmatrix} a_{11} & \cdots & a_{1m} \\ \vdots & \ddots & \vdots \\ a_{m1} & \cdots & a_{mm} \end{pmatrix} + \frac{1}{\sqrt{s}} \begin{pmatrix} \sigma_{11}\xi_{11} & \cdots & \sigma_{1m}\xi_{1m} \\ \vdots & \ddots & \vdots \\ \sigma_{m1}\xi_{m1} & \cdots & \sigma_{mm}\xi_{mm} \end{pmatrix}, \tag{80}$$

where $\xi_{ij}$ for all $i$ and $j$ are independent random variables with mean 0 and variance 1. In this case, we can simplify the system equation:

$$\dot{x}_i = sx_i \left[\pi_i - \bar{\pi} + (Y^T\Sigma Y - (\Sigma Y)_i x_i) + \frac{1}{2}((\Sigma Y)_i - X^T\Sigma Y)\right], \tag{81}$$

where

$$\Sigma = \begin{pmatrix} \sigma_{11}^2 & \cdots & \sigma_{1m}^2 \\ \vdots & \ddots & \vdots \\ \sigma_{m1}^2 & \cdots & \sigma_{mm}^2 \end{pmatrix}, \tag{82a}$$

$$X = [x_1, x_2, \cdots, x_m]^T, \tag{82b}$$

$$Y = [x_1^2, x_2^2, \cdots, x_m^2]^T, \tag{82c}$$

and $(\Sigma Y)_i$ represents the $i_{th}$ element of vector $\Sigma Y$. Particularly, for two-strategy games, Eq. 81 simplifies to

$$\dot{x} = sx(1-x)\left[\pi_C - \pi_D + (\frac{1}{2} - x)\left((\sigma_a^2 + \sigma_c^2)x^2 + (\sigma_b^2 + \sigma_d^2)(1-x)^2\right)\right]. \tag{83}$$

We can find that this equation actually has similar properties as the case of a single noise source (Eq. 20), where the environmental fluctuations are always beneficial for cooperators when $x < 1/2$ and beneficial for defectors when $x > 1/2$.

For Eq. 83, even if we assume $\sigma_a = ka$ (the same for $\sigma_b$, $\sigma_c$ and $\sigma_d$), we can no longer use only two parameters to categorize its dynamical patterns. Thus, it is complicated to explore the parameter region for all dynamical patterns like Figure 3 in the main text. We only investigate some specific games to show that in this case, environmental fluctuations can also reshape the game dynamics and the dynamical patterns are similar to the scenario of a single noise source (see Supplementary Fig. 9). These results remain qualitatively consistent with the case of the single noise source.

Similarly, we also explore the RPS games under this setting (i.e., $A_{ij} = a_{ij} + ka_{ij}\xi_{ij}/\sqrt{s}$). The results are also consistent with the single noise case. For $\beta > \alpha$, $k > 0$ can also induce a stable limit cycle. For $\beta \leq \alpha$, the environmental fluctuations also accelerate the convergence of the trajectories towards the central equilibrium $e^*$ (Supplementary Fig. 10).

### 3.2.2 Colored noise

In the above discussion, the noise $\xi$ in each time step is independent (i.e., the noise is white). In each generation, $\xi$ will be randomly sampled which is independent of the previous environment state (the value of $\xi$). In other words, the environment fluctuates very rapidly. However, in many real cases, the environmental noise between two generations may not be independent. The environment state may memorize partial information of the previous states (i.e., the noise is colored).

Let $\xi_\tau$ denote the random variable in generation $\tau$. Then, we assume that the environmental noise obeys the following properties:

(1) The stationary distribution of $\xi_\tau$ still obeys a normal distribution $\mathcal{N}(0,1)$.

(2) $\xi_\tau$ is a Markov process.

(3) The correlation coefficient of two generations $\xi_\tau$ and $\xi_{\tau+1}$ is $\rho(\xi_\tau,\xi_{\tau+1}) = 1-\nu$, i.e., $\mathrm{Cov}(\xi_\tau,\xi_{\tau+1}) = 1-\nu$.

Here, $0 < \nu \leq 1$ is satisfied. Condition (3) implies that in each time step, the environment state will retain the fraction $1-\nu$ of the information of the previous environment state, and the rest fraction $\nu$ is contributed by new fluctuation. Note that $\nu$ describes the speed of environmental fluctuations relative to that of strategy evolution. A small correlation (large $\nu$) means the noise between each two generations is nearly independent, which implies the environment fluctuates quickly. Whereas a large correlation (small $\nu$) implies the environment fluctuates slowly. For a special case, if $\nu = 0$, the environment state is constant.

If $\nu = 1$, the environmental noise in each time step is independent, which simplifies to the case of white noise discussed above. And $\nu \to 0$ corresponds to the case that the environment fluctuates very slowly compared with the change of strategy frequency. When $0 < \nu < 1$, the noise is intermediate between white and quenched.

A widely used process to model the environmental fluctuations under colored noise is the auto-regressive (AR) process [7]. We assume that in time step $\tau+1$, $\xi_{\tau+1}$ will retain a partial information of $\xi_\tau$ with the fraction of $1-\nu$, which implies

$$\xi_{\tau+1} = (1-\nu)\xi_\tau + \sqrt{1-(1-\nu)^2}\eta = (1-\nu)\xi_t + \sqrt{2\nu-\nu^2}\eta. \tag{84}$$

Here, $\eta$ is a standard Gaussian random variable which is independent in different time steps. We can check that if $\xi_\tau \sim \mathcal{N}(0,1)$, $\xi_{\tau+1}$ also obeys a standard normal distribution. Actually, $\mathcal{N}(0,1)$ (the normal distribution with mean 0 and variance 1) is the stationary distribution of $\xi_t$. Similarly, to ensure the timescale corresponds to the replicator equation (see Section 2.1.1), we still introduce the notation $t = \tau/N$. And Eq. 84 becomes

$$\xi_{t+1/N} = (1-\nu)\xi_t + \sqrt{2\nu-\nu^2}\eta. \tag{85}$$

Then, the correlation function of $\xi_t$ is

$$\mathrm{Cov}(\xi_t,\xi_{t+\Delta t}) = \mathbb{E}[\xi_t\xi_{t+\Delta t}] = (1-\nu)^{N\Delta t}. \tag{86}$$

We define $\delta = \nu N$. Then,

$$Cov(\xi_t,\xi_{t+\Delta t}) = \mathbb{E}[\xi_t\xi_{t+\Delta t}] = (1-\delta/N)^{N\Delta_t} \approx \exp(-\delta\Delta t). \tag{87}$$

We analyze two limit cases. For colored noise, there is no modified replicator equation (ODE) to describe the system dynamics. Thus, we focus on the stationary distribution of $x$, denoted by $\upsilon(x)$. To avoid absorption, we adopt a technical assumption that the boundary is reflecting, which means that if cooperators/defectors become extinct, another new cooperator/defector will emerge instantly.

If $\nu \gg 1/N$ (i.e. $\delta \gg 1$), the correlation function decays exponentially and tends to zero. Thus, the average memory time of the environment state is very short, such that it can be regarded as the memory-less case (i.e., white noise). For two strategy games in this case, the stationary distribution will show humps in the stable equilibrium points of replicator equation Eq. 20. Thus, for wide range

of values of $\nu$ (i.e., $\nu \gg 1/N$), the system dynamics remains qualitatively the same as the case of white noise, which can be well described by Eq. 20.

If $\nu \ll 1/N$, the environment changes very slowly such that the population composition $x$ equilibrates much more quickly than the environment states. For a fixed environment state (a fixed value of $\xi$), the system will evolve according to the classic replicator equation

$$\dot{x} = sx(1-x)(\Pi_C - \Pi_D), \tag{88}$$

where $\Pi_C$ and $\Pi_D$ are defined in Eq. 2 (but here $\xi$ is regarded as a constant). Thus, the system can be regarded as moving on the curve which is constituted of stable equilibrium points of Eq. 88 for all values of $\xi$. Suppose the environmental noise $\xi$ is fixed with value $\lambda$. This equilibrium curve $x^*(\lambda)$ is the stable equilibrium of the following payoff matrix:

$$A = \begin{pmatrix} A_{11} & A_{12} \\ A_{21} & A_{22} \end{pmatrix} = \bar{A} + \frac{\lambda}{\sqrt{s}}\Sigma = \begin{pmatrix} a & b \\ c & d \end{pmatrix} + \frac{\lambda}{\sqrt{s}} \begin{pmatrix} \sigma_a & \sigma_b \\ \sigma_c & \sigma_d \end{pmatrix} \tag{89}$$

Note that this $x^*(\lambda)$ function may be multivalued. If the perturbed game is a prisoner's dilemma game (i.e., $A_{11} < A_{21}$ and $A_{12} < A_{22}$), $x^*(\lambda) = 0$ always hold. If the perturbed game is a snowdrift game (i.e., $A_{11} < A_{21}$ and $A_{12} > A_{22}$), $x^*(\lambda)$ is

$$x^*(\lambda) = \frac{\sqrt{s}(d-b) + (\sigma_d - \sigma_d)\lambda}{\sqrt{s}(a-b-c+d) + (\sigma_a - \sigma_b - \sigma_c + \sigma_d)\lambda}. \tag{90}$$

If the perturbed game is a coordination game (i.e., $A_{11} > A_{21}$ and $A_{12} < A_{22}$), $x^*(\lambda)$ equals 1 and 0 (multivalued). Formally, the stationary distribution of $x$ can be expressed as

$$p(\lambda^{-1}(x^*))\frac{\mathrm{d}\lambda}{\mathrm{d}x^*} \tag{91}$$

where $p(\lambda)$ is the stationary distribution of the AR process (i.e, standard normal distribution) and $\lambda^{-1}(x^*)$ is the inverse function of $x^*(\lambda)$.

In one special case that we have considered previously, when the noise intensity is proportional to the mean payoff, the payoff structure becomes,

$$A = \left(1 + \frac{k\lambda}{\sqrt{s}}\right)\begin{pmatrix} a & b \\ c & d \end{pmatrix} \tag{92}$$

If $1 + \frac{k\lambda}{\sqrt{s}} > 0$, this game has the same stable equilibrium as the mean payoff matrix $[a,b;c,d]$. But when $1+\frac{k\lambda}{\sqrt{s}} < 0$, this game has the same equilibrium as the opposite mean payoff matrix as $-[a,b;c,d]$. Since $\lambda$ obeys the normal distribution, $1+\frac{k\lambda}{\sqrt{s}}$ can either be positive or negative for different noise value $\lambda$. For example, as seen in Supplementary Fig. S11, for the quenched noise limit (panel d and h), the stationary distribution has humps on the boundary $x = 0$ and $x = 1$ (which are stable equilibrium of the mean payoff matrix $\bar{A}$) and $x = 1/3$ (which is the stable equilibrium of the payoff matrix $-\bar{A}$).

For the proportional noise case, we give an example of evolutionary trajectories and the stationary distribution (Supplementary Fig. 11) for different correlation strength ($\nu$). We also provide a parallel version of Fig. 3b for the quenched noise limit ($\nu \to 0$, see Supplementary Fig. 12). In this case, the noise intensity is proportional to the mean payoff. For a prisoner's dilemma $\bar{A}$, $-\bar{A}$ is a harmony game ($x = 1$ is the unique stable equilibrium). If $\bar{A}$ is a snowdrift game, $-\bar{A}$ is a coordination game. Thus,

for both harmony game and prisoner's dilemma, the stationary distribution with strongly correlated environmental noise has the property that there are two humps, at $x = 0$ and $x = 1$. For both snowdrift game and coordination game, the stationary distribution looks has three humps, at $x = 0$, $x = x^* = \frac{d-b}{a-b-c+d}$ and $x = 1$.

We also provide an example when noise is not proportional to the mean payoff in the regime $\nu \to 0$ (quenched noise limit). In this case, the stationary distribution is given by Eq. 91 (see Supplementary Fig. 13).

### 3.3 Small populations: fixation probability

Our model is described by a discrete Markov chain, where full cooperation and full defection are the only absorbing states. A population starting from any initial configuration will eventually converge to one of these two states, through a combination of selection induced by deterministic payoff differences, noise in payoffs, and demographic stochasticity. But if the population size is large, the expected fixation time is extremely large (actually exponential in the population size), which has led to to focus on interior dynamics neglecting demographic stochasticity.

In this section, we also consider small populations subject to demographic stochasticity, where all interior equilibrium structure vanishes and the dynamics are described by fixation probabilities of one type or another. The fixation probability for cooperators is the probability that a single mutant of cooperator can invade and take over the whole population otherwise full of defectors. And the fixation probability for defectors can be defined similarly. The fixation probability can be studied analytically by using the method of Fudenberg and Imhof [8]. The fixation probability of cooperators is

$$\rho = \frac{1}{1 + \sum\limits_{k=1}^{N-1} \prod\limits_{i=1}^{k} \frac{T^-(i)}{T^+(i)}}, \tag{93}$$

where $T^+(i)$ and $T^-(i)$ is given by Eq. 4.

Given Eq. 8, the fixation probability can also be approximated by [9]

$$\rho_C \approx \frac{\int_0^{\frac{1}{N}} \left( \exp \int^y - \frac{2a(z)}{b(z)^2} \mathrm{d}z \right) \mathrm{d}y}{\int_0^1 \left( \exp \int^y - \frac{2a(z)}{b(z)^2} \mathrm{d}z \right) \mathrm{d}y}, \tag{94}$$

where $a(x) = T^+(x) - T^-(x)$ and $b(x) = \sqrt{[T^+(x) + T^-(x)]/N}$. Here we consider two scenarios, one is the single noise source case, and the other is that each element of the payoff matrix is subject to independent noise.

**(A) Single noise source**

We first consider the single noise case, namely, the payoff structure is

$$\Pi = \bar{\Pi} + \xi\Sigma = \begin{bmatrix} a & b \\ c & d \end{bmatrix} + \frac{\xi}{\sqrt{s}} \begin{bmatrix} \sigma_a & \sigma_b \\ \sigma_c & \sigma_d \end{bmatrix}. \tag{95}$$

In this case, according to Eq. 20 and Eq. 15b, $a(x)$ and $b(x)$ are given by

$$a(x) = sx(1-x)[\pi_C - \pi_D + (1/2 - x)(\sigma_C - \sigma_D)^2], \tag{96a}$$

$$b(x) = \sqrt{2x(1-x)/N}. \tag{96b}$$

Under weak selection ($s \ll 1$), we can expand the fixation probability to the first order of $s$:

$$\begin{aligned}\rho_C &= \frac{\int_0^{1/N}\left(\exp\int^y -sN[\pi_C-\pi_D+(\frac{1}{2}-x)(B_\sigma+(A_\sigma-B_\sigma)x)^2]\mathrm{d}x\right)\mathrm{d}y}{\int_0^1\left(\exp\int^y -sN[\pi_C-\pi_D+(\frac{1}{2}-x)(B_\sigma+(A_\sigma-B_\sigma)x)^2]\mathrm{d}x\right)\mathrm{d}y} \\ &= \frac{1}{N}+s\left(\frac{B_\sigma^2}{12}-\frac{(A_\sigma-B_\sigma)^2}{120}+\frac{1}{6}(a-c)+\frac{1}{3}(b-d)\right)+o(s),\end{aligned} \tag{97}$$

where $A_\sigma=\sigma_a-\sigma_c$ and $B_\sigma=\sigma_b-\sigma_d$.

Similarly, the fixation probability of defectors is

$$\begin{aligned}\rho_D &= \frac{\int_{1-1/N}^{1}\left(\exp\int^y -sN[\pi_C-\pi_D+(\frac{1}{2}-x)(B_\sigma+(A_\sigma-B_\sigma)x)^2]\mathrm{d}x\right)\mathrm{d}y}{\int_0^1\left(\exp\int^y -sN[\pi_C-\pi_D+(\frac{1}{2}-x)(B_\sigma+(A_\sigma-B_\sigma)x)^2]\mathrm{d}x\right)\mathrm{d}y} \\ &= \frac{1}{N}+s\left(\frac{A_\sigma^2}{12}-\frac{(A_\sigma-B_\sigma)^2}{120}-\frac{1}{6}(b-d)-\frac{1}{3}(a-c)\right)+o(s).\end{aligned} \tag{98}$$

Cooperation is favored by natural selection when the stationary frequency of cooperators is higher than 1/2. If the mutations are rare, it is equivalent to $\rho_C>\rho_D$ [8]. That is

$$(\sigma_b-\sigma_d)^2-(\sigma_a-\sigma_c)^2>-6(a+b-c-d), \tag{99}$$

We can find that the fixation probability only depends on $\sigma_b-\sigma_d$ and $\sigma_a-\sigma_c$. We also perform simulations for the donation game to verify our analysis here (Supplementary Fig. 1).

**(B) Independent noise sources**

Next, as in Section S3.2.1, we consider the case that the noise of each element in payoff is independent. The payoff structure is given by

$$\Pi=\begin{bmatrix} a & b \\ c & d\end{bmatrix}+\frac{1}{\sqrt{s}}\begin{bmatrix}\sigma_a\xi_a & \sigma_b\xi_b \\ \sigma_c\xi_c & \sigma_d\xi_d\end{bmatrix}. \tag{100}$$

Under this assumption, using similar techniques, we can obtain $a(x)$ and $b(x)$:

$$a(x)=sx(1-x)[\pi_C-\pi_D+(1/2-x)((\sigma_a^2+\sigma_c^2)x^2+(\sigma_b^2+\sigma_d^2)(1-x)^2)], \tag{101a}$$

$$b(x)=\sqrt{2x(1-x)/N}. \tag{101b}$$

The fixation probabilities for cooperators and defectors are approximated by

$$\rho_C=\frac{1}{N}+s\left[\frac{1}{6}(a-c)+\frac{1}{3}(b-d)+\frac{9}{120}(\sigma_b^2+\sigma_d^2)-\frac{1}{120}(\sigma_a^2+\sigma_c^2)\right]+o(s), \tag{102a}$$

$$\rho_D=\frac{1}{N}+s\left[-\frac{1}{6}(b-d)-\frac{1}{3}(a-c)+\frac{9}{120}(\sigma_a^2+\sigma_c^2)-\frac{1}{120}(\sigma_b^2+\sigma_d^2)\right]+o(s). \tag{102b}$$

Then, the condition $\rho_C>\rho_D$ simplifies to

$$(\sigma_b^2+\sigma_d^2)-(\sigma_a^2+\sigma_c^2)>-6(a+b-c-d). \tag{103}$$

Note that in these two condition Eq. 99 and Eq. 103, $\sigma_a,\cdots,\sigma_d$ are rescaled by $\sqrt{s}$. Thus, for a fixed intensity of fluctuation ($\tilde{a},\cdots,\tilde{d}$), the selection intensity can also affect the evolution of cooperation. Specifically, if $(\tilde{b}-\tilde{d})^2-(\tilde{a}-\tilde{c})^2>0$ in Eq. 99 or $(\tilde{b}^2+\tilde{d}^2)-(\tilde{a}^2+\tilde{c}^2)>0$, larger selection intensity always makes these two conditions easier to be satisfied, which is beneficial for the evolution of cooperation. This result seems contradicts to the classic results. Prior studies often show that in a prisoner's dilemma, larger selection intensity is always detrimental to cooperators' evolution.

Furthermore, Eq. 20 shows that for large populations, the stable equilibrium can never be greater than 1/2 in the prisoner's dilemma game (where $\pi_C - \pi_D$ is always negative). That is, the equilibrium frequency of cooperators can never exceed defectors for any noise structures. However, for a small population, the stationary frequency of cooperators can exceed defectors when Eq. 99 or Eq. 103 holds. This is because in a large population, only environmental noise can affect the dynamics. But for small populations, demographic noise also matters. Even though demographic noise alone cannot make cooperation favored, a combination of demographic and environmental noise can.

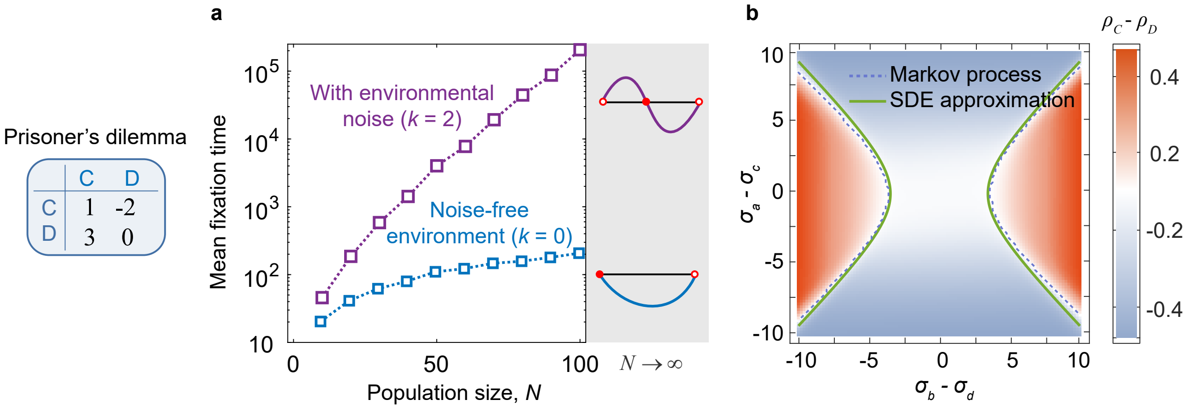


Supplementary Fig 1: **Fixation probability and fixation time for prisoner's dilemma.** Here we consider small populations. In small populations, demographic noise cannot be ignored. The system will finally enter the two absorbing states: full cooperation or full defection. Assume that there is only one cooperator in the population and all the other individuals are defectors. The probability that the cooperator can take over the whole population is called the fixation probability of cooperators (denoted by $\rho_C$). Similarly, the fixation probability of defectors is denoted by $\rho_D$. The average fixation time is the average number of generations when cooperators fix or defectors fix. Here we consider a prisoner's dilemma game. (**a**) Compared with the noise-free environment ($k = 0$), the fixation time in a noisy environment is far longer. Intuitions can also be found in our modified system equation Eq. 20 (large population limit). In the noisy environment, there is an interior stable equilibrium, which makes the population much harder to fix on the boundary, especially when the population size is large (where the demographic noise can be ignored). This means that when the population is large, the system will stay around the coexistence equilibrium for an extremely long time before it fixes. (**b**) For a fixed population, different environmental noise structures can affect the fixation probabilities. For the prisoner's dilemma considered here, we compute the accurate fixation probability (for the Markov birth-death process) by Eq. 93. The red region represents that cooperation can evolve (i.e., $\rho_C > \rho_D$), which is impossible if environment noise is absent and without other mechanisms. The critical line (dashed line) is also illustrated. And the fixation probability can also be approximated by the SDE (see Eq. 97). According to the approximated fixation probability, we can also give an approximation for the critical line (solid line), which is $(\sigma_b - \sigma_d)^2 - (\sigma_a - \sigma_c)^2 = -12$ (see Eq. 99). These results show that environmental noise still has great influences on evolutionary dynamics even for small populations. Parameters: $s = 0.1$, $N = 100(b)$.

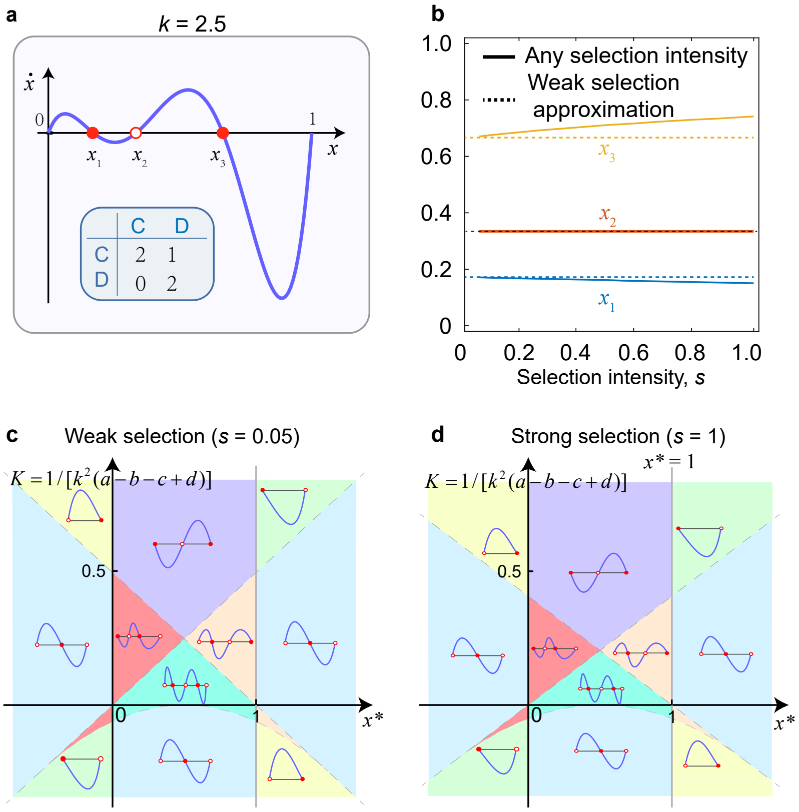


Supplementary Fig 2: **Replicator equation provides good approximations for dynamical patterns under strong selection.** For weak selection ($s \ll 1$), we derive the replicator equation (Eq. 20) to solve the equilibrium explicitly. Here, we show that the equilibrium solutions of the replicator equation are still good approximations for a wide range of selection intensities. (**a**) We choose a coordination game $\bar{A} = [2, 1; 0, 2]$ as an example (the example in Fig. 2f in the main text). For noise intensity $k = 2.5$, the solution of the replicator equation is shown in (**a**). The three interior equilibrium points are denoted by $x_1$, $x_2$, $x_3$. For different selection intensities, we compute the precise interior equilibrium points shown in **b**. As the selection intensity increases, the number of equilibrium points remains invariant, and the actual values of equilibrium points vary not much compared with the prediction from the replicator equation, even for strong selection intensity. (**c, d**) We compute the precise spectrum of the dynamical patterns by simulation (simulated versions of Fig. 3b in the main text). For weak selection, the spectrum agrees well with our prediction (Fig. 3b) by the replicator equation (Eq. 20). For strong selection, it still remains qualitatively consistent with Fig. 3b, with a slight compression in the $K$-axis. These results show that the replicator equation derived for weak selection still serves as a decent approximation for strong selection.

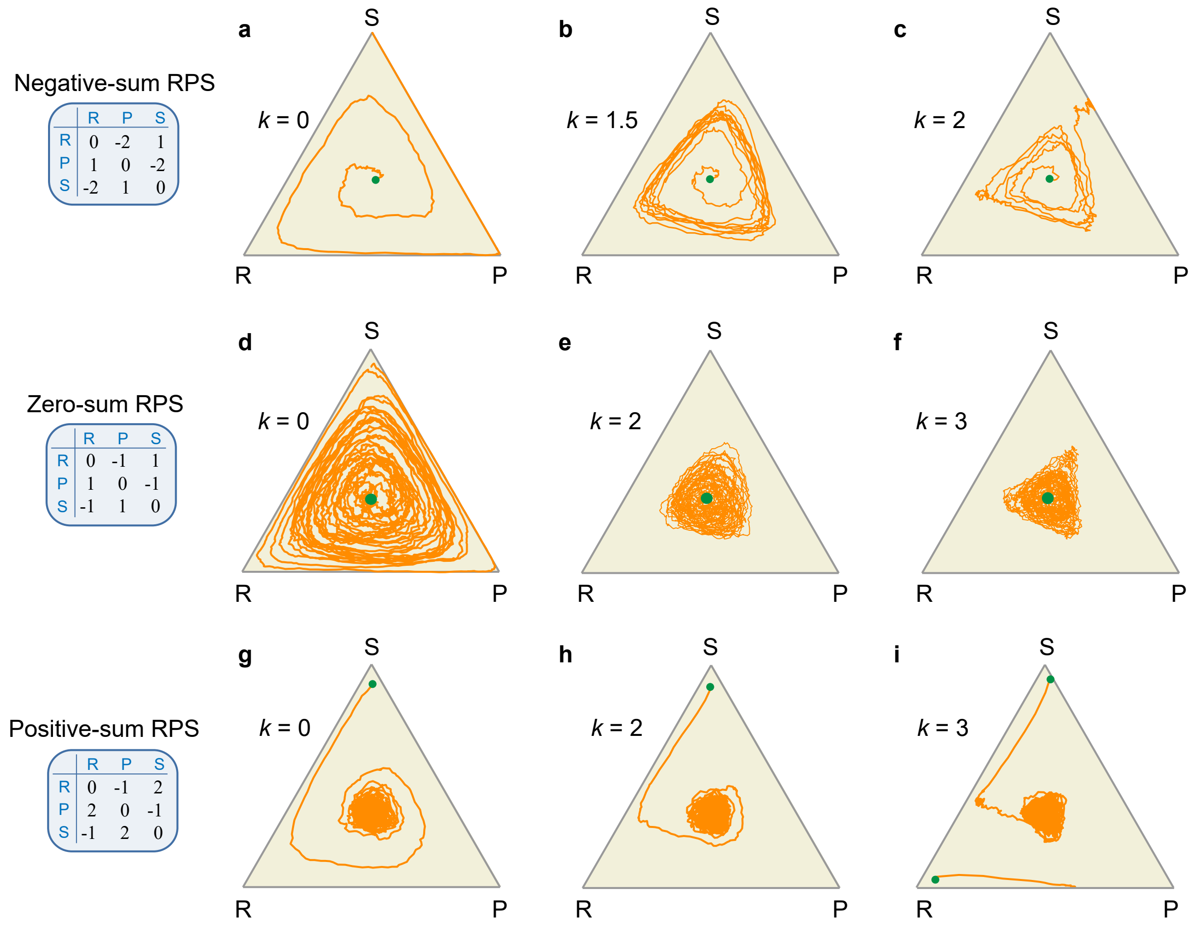


Supplementary Fig 3: **Simulated trajectories for rock-paper-scissors games under noisy environment.** We perform Monte-Carlo simulations in a finite population to verify the theoretical predictions in Fig. 4 of the main text. Each trajectory (yellow lines) starts from the green point. By simulation we see that for the negative-sum RPS game (**a**) environmental fluctuations can induce stable limit cycles (**b, c**), enabling the coexistence of the three types. For the zero-sum RPS game, simulations show that the environmental fluctuations tend to stabilize the trajectories around the center (**e, f**), which is stable but not attractive if noise is absent (**d**). For a positive-sum RPS game, although the center of the simplex is asymptotically stable in noise-free environment (**g**), fluctuations can still accelerate the convergence to the center (**h, i**). Parameters: $s = 0.1, N = 20000$.

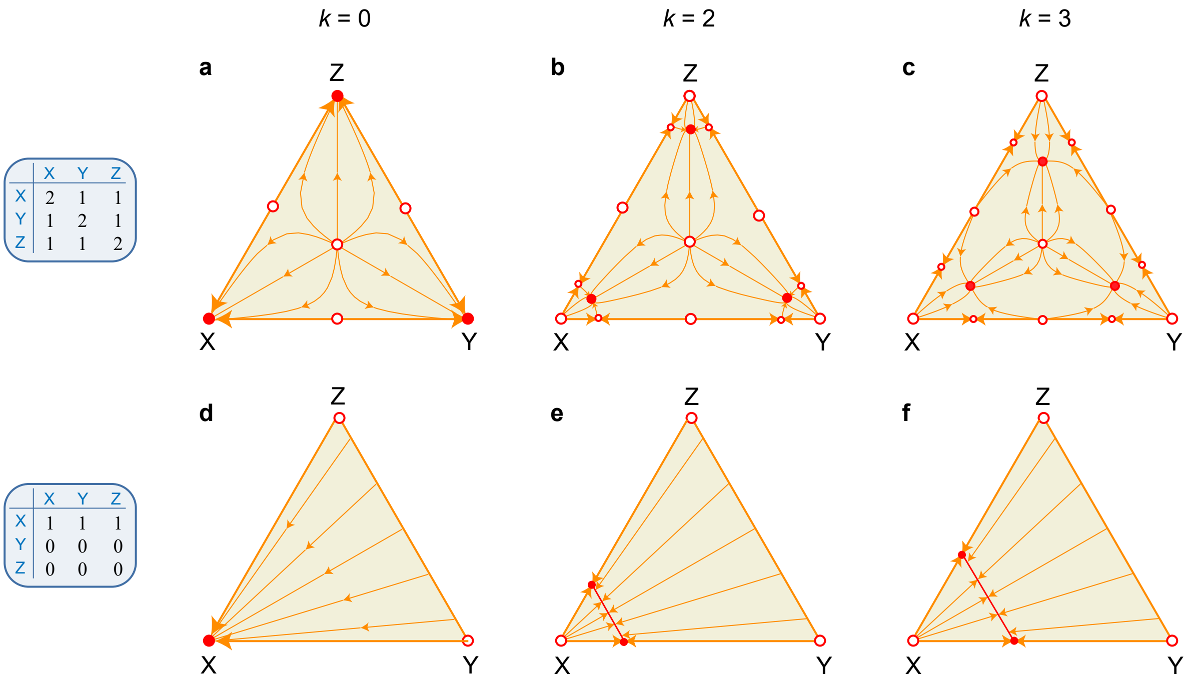


Supplementary Fig 4: **Dynamical patterns for other types of three-strategy games with environmental fluctuations.** We also investigated the population dynamics of several other three-strategy games. Here, we consider two classes of games: each strategy is self-dominated (**a, b, c**), and one strategy always dominates another two strategies (**d, e, f**). Environmental fluctuations can still induce more interior stable equilibrium points, and the dynamical patterns also become more complicated. Parameter: $s = 0.1$

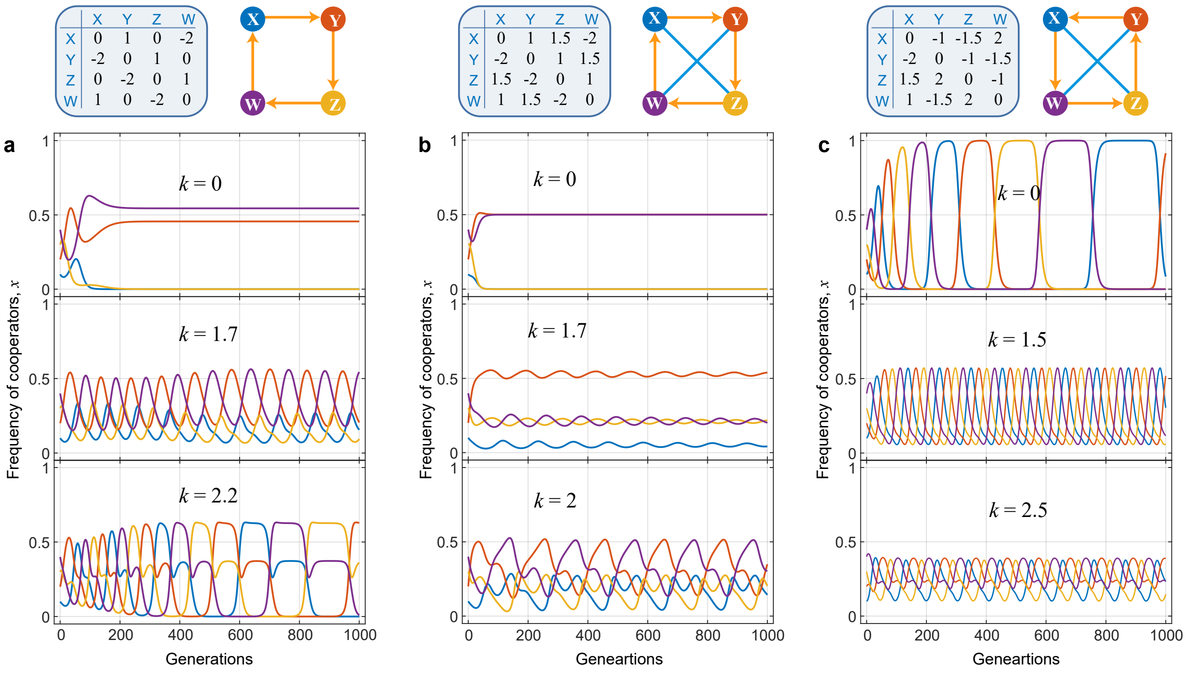


Supplementary Fig 5: **Environmental fluctuations can strengthen coexistence of strategies in four-strategy games.** We also study evolutionary dynamics in games with four strategies. Like RPS games, we assume that there are no dominant strategies. Each strategy dominates one strategy and is also dominated by another strategy circularly. We illustrate three examples of four-strategy games. The arrows indicate the dominance relation between strategies. For all the three examples, a noisy environment can yield oscillating evolution trajectories of different strategies. All strategies coexist without extinction, which does not occur in a noise-free environment ($k = 0$). Parameters: $s = 0.1$, initial frequencies of the four strategies: $x_1 = 0.1, x_2 = 0.2, x_3 = 0.3, x_4 = 0.4$

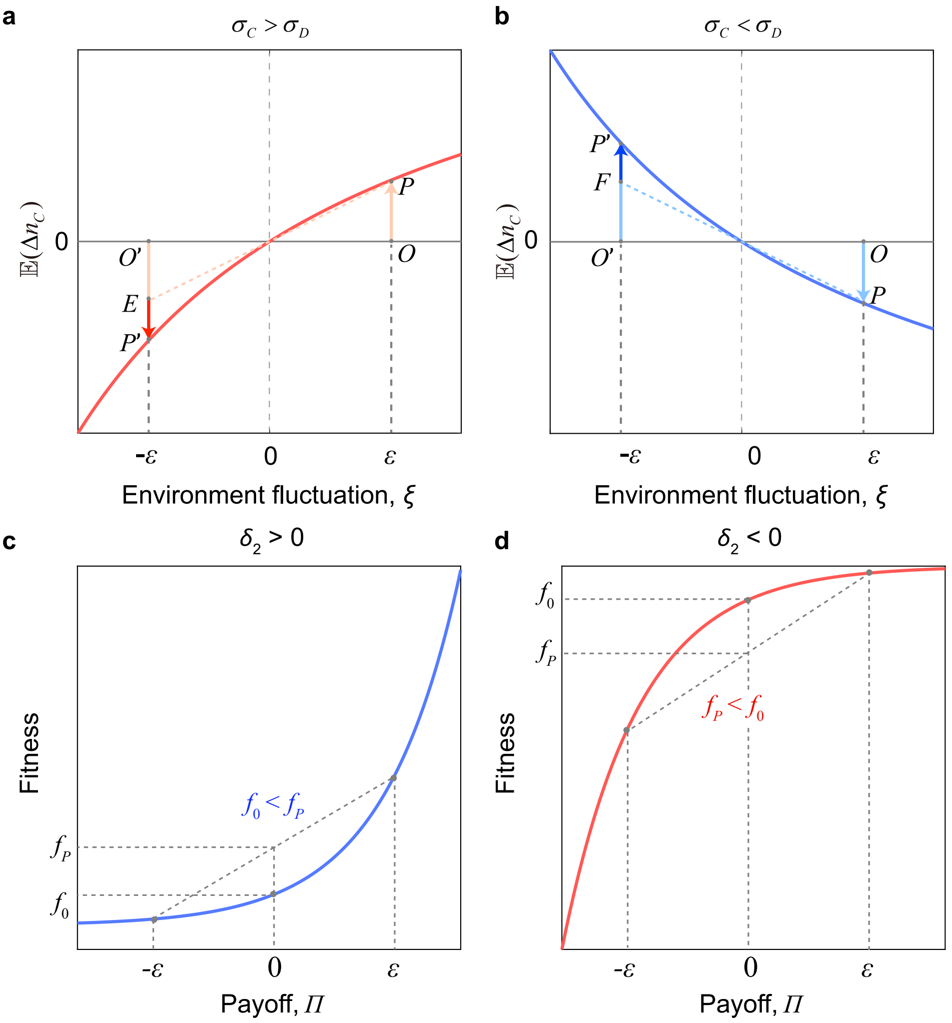


Supplementary Fig 6: **Illustration of effects of noise including general fitness functions.** As discussed in the main text, the effects of environment fluctuations on the evolutionary dynamics arise from two factors: non-linear updating rules and non-linear payoff-to-fitness function. **a, b**, The expected change in the number of cooperators for symmetric environmental fluctuations and a linear fitness function $f_i = 1 + s\Pi_i$. We assume that individuals' baseline payoffs are zero, and then the actual payoffs are determined by the fluctuations (i.e., $\Pi_C = \sigma_C \xi/\sqrt{s}$ and $\Pi_D = \sigma_D \xi/\sqrt{s}$). For symmetric fluctuations, the environment state transitions to $\xi$ equals $\epsilon$ and $-\epsilon$ with the same probability. If fluctuations are more intense for cooperators' payoffs ($\sigma_C > \sigma_D$) (**a**), perturbations $\xi = \epsilon$ leads to an increase in the number of cooperators by $OP$, and perturbations $\xi = -\epsilon$ leads to a decrease in the number of cooperators by $OP'$. Nonetheless the two effects are not symmetric, which yields a net decrement in the number of cooperators, by $EP'$. Similarly, if defectors' payoffs fluctuate more intensively, a symmetric fluctuation yields a net increment in cooperators (**b**). **c, d**, The expected change in the number of cooperators for a non-linear fitness function. The baseline (deterministic) payoffs are zero. **c**, If the fitness function is convex ($\delta_2 > 0$), a payoff with less fluctuation (for example, payoff 0 deterministically) generates a lower expected fitness than a payoff with stronger fluctuation (for example, $-\epsilon$ or $\epsilon$ with identical probability). **d**, Conversely, when the fitness function is concave ($\delta_2 < 0$) a payoff with lower fluctuation generates higher expected fitness.

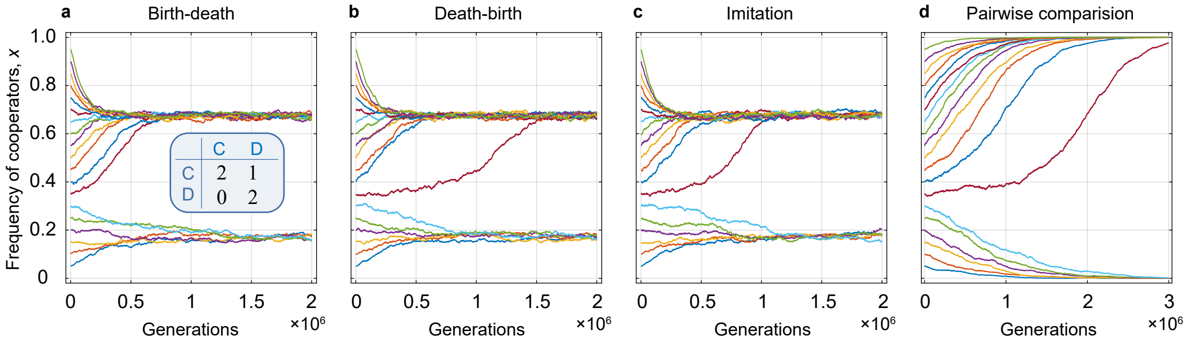


Supplementary Fig 7: **Evolutionary dynamics under different updating rules.** We consider an example when the deterministic component of the payoff structure is $\bar{A} = [2, 1; 0, 2]$ (coordination game). In the noise-free case, there are only two stable equilibria, on the boundary $x = 0$ or $x = 1$. When the environment is subject to stochastic fluctuations, under birth-death, death-birth, and imitation process, there are two stable equilibrium points which are in the interior and therefore support a mixture of types. The locations of the equilibria and their stabilities are identical for the first three updating rules (**a, b, c**). However, for the pairwise comparison rule, the dynamics are the same as in the noise-free case, which means that stochastic fluctuations have no effect on the dynamics under pairwise comparison rule (**d**). Parameters: $s = 0.1$, $N = 20000$, $k = 2.5$.

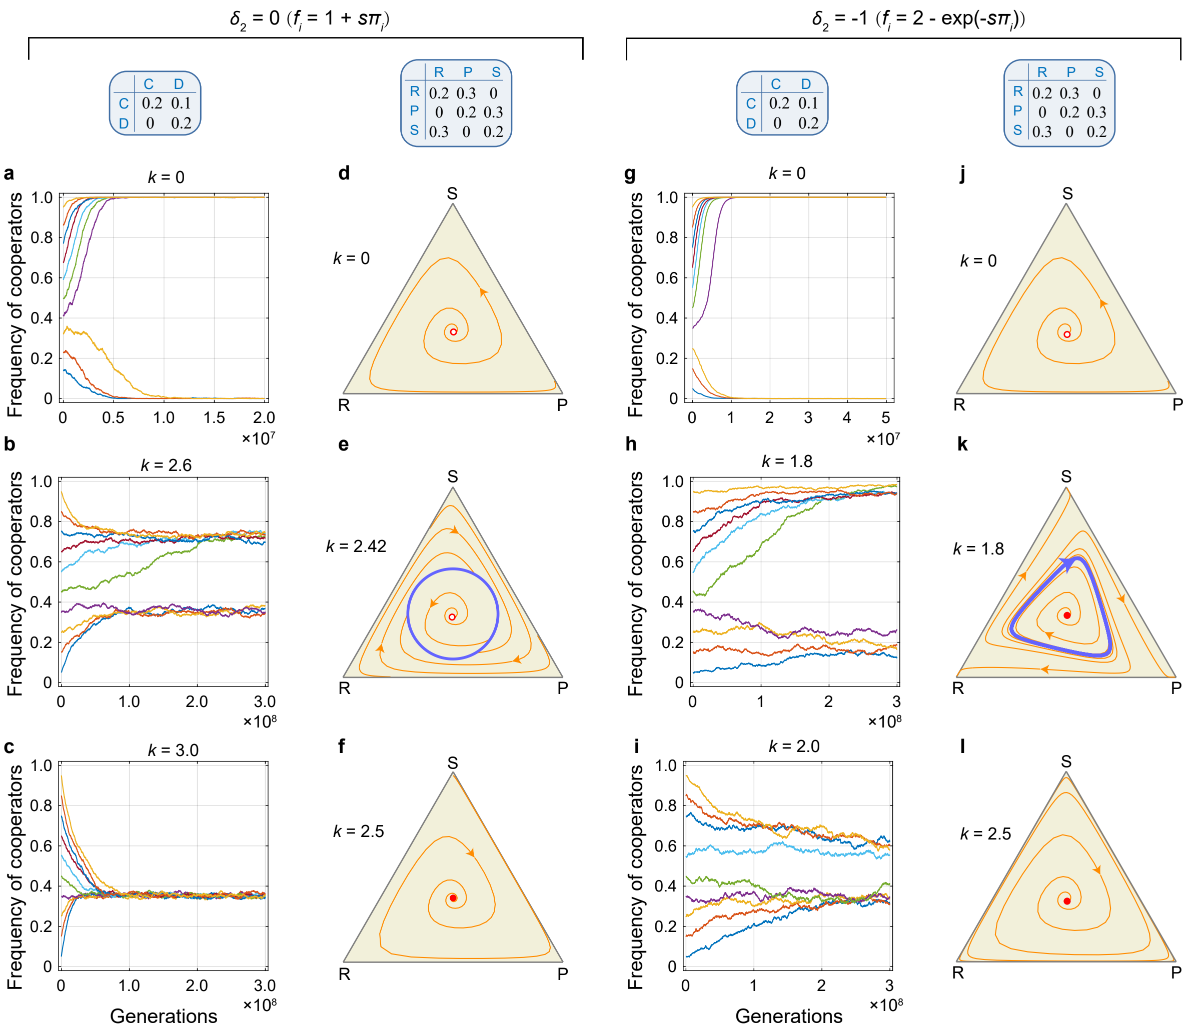


Supplementary Fig 8: **Dynamical patterns for different fitness functions.** According to the analysis in section 3.1, the fitness function $f_i = f(s\Pi_i)$ can be categorized into three types: $\delta_2 > 0$, $\delta_2 = 0$, $\delta_2 < 0$ where $\delta_2 = f''(0)/f'(0)$. Apart from the classic exponential fitness function ($f_i = \exp(s\pi_i)$) where $\delta_2 = 1 > 0$, we also consider two other kinds of fitness function where $\delta_2 = 0$ (**a-f**) and $\delta_2 < 0$ (**g-l**). We choose a representative two-strategy game (stag-hunt) and an RPS game to illustrate the resulting dynamical patterns. In all cases, environmental noise can induce more equilibria in the interior, supporting a stable diversity of types. Periodic obits also emerge in RPS games for intermediate noise intensity. These results remain qualitatively consistent with Fig. 2 and Fig. 4 in the main text. Parameters: $s = 0.1, N = 20000$.

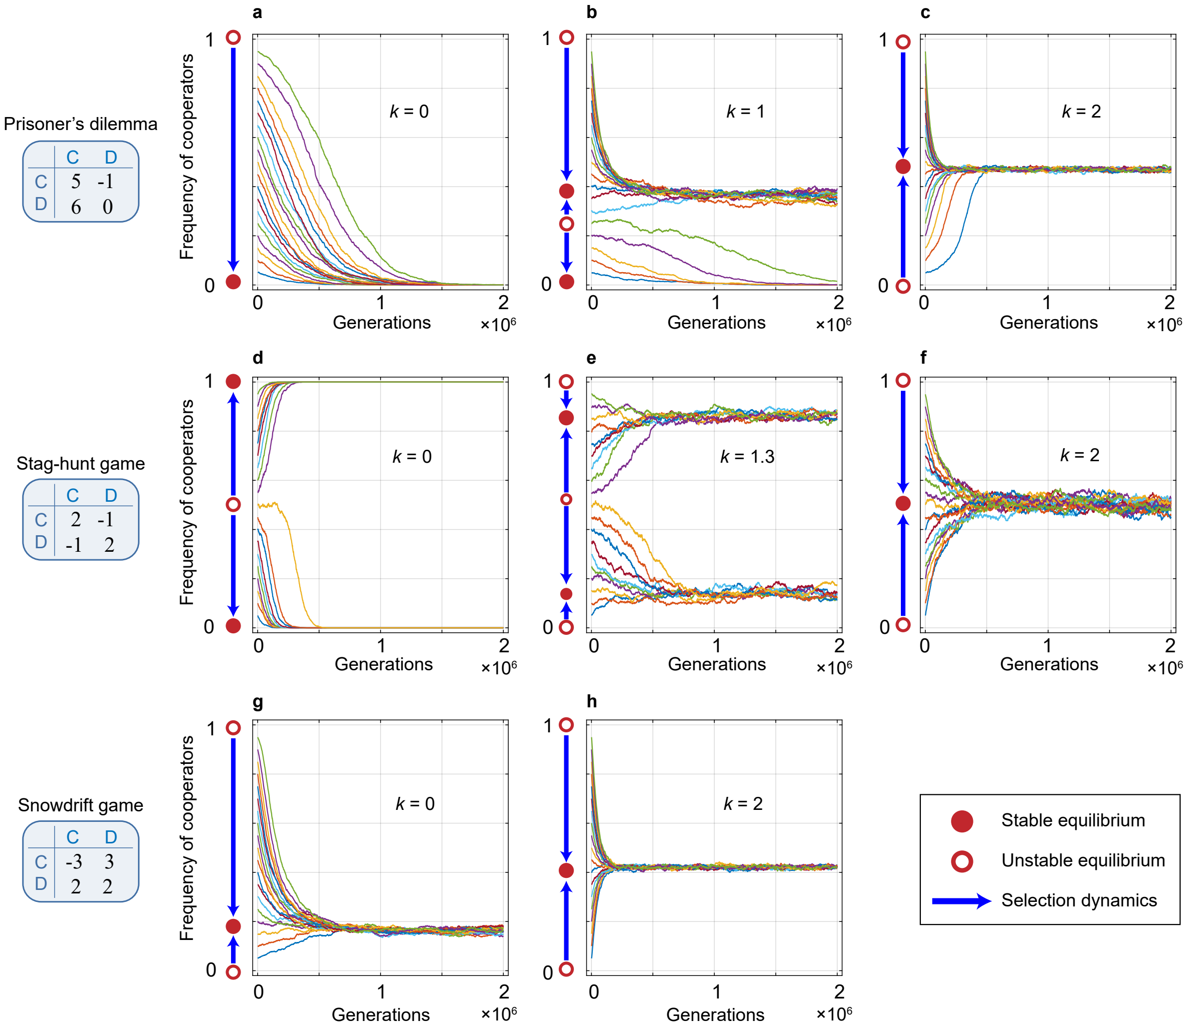


Supplementary Fig 9: **Evolutionary dynamics of two-strategy games under independent environmental noise.** In the main text, we assume that the fluctuations are controlled by a single random variable $\xi$. Here, we assume that each element in the payoff matrix is subject to an independent noise, and the intensity of the noise is proportional to the baseline payoff matrix (with coefficient $k$, Eq. 80). Thus for a two-strategy game, the fluctuations are controlled by four independent random variables. The blue arrows and red points represent the analytic results obtained from the system equation (Eq. 83). All trajectories with different initial configurations are obtained by Monte-Carlo simulations. For different types of games, the environmental fluctuations can still lead to more complicated patterns, including two interior stable equilibria (**e**), two stable equilibria with one on the boundary and the other in the interior (**b**). These results remain qualitatively consistent with the correlated noise case (Fig. 2 in the main text). Parameters: $N = 20000$, $s = 0.1$.

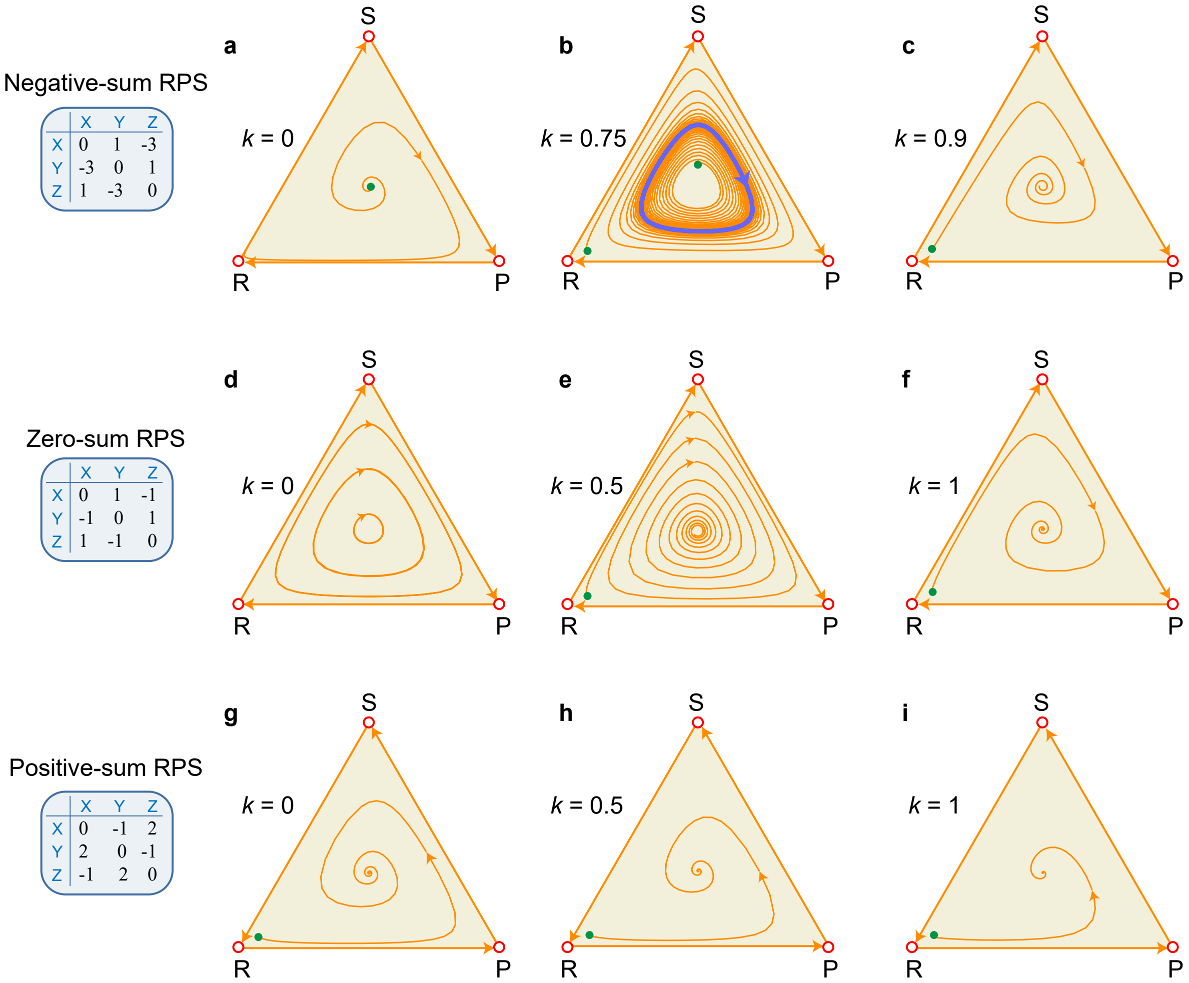


| | X | Y | Z |
|---|---|---|---|
| X | 0 | 1 | -3 |
| Y | -3 | 0 | 1 |
| Z | 1 | -3 | 0 |

| | X | Y | Z |
|---|---|---|---|
| X | 0 | 1 | -1 |
| Y | -1 | 0 | 1 |
| Z | 1 | -1 | 0 |

| | X | Y | Z |
|---|---|---|---|
| X | 0 | -1 | 2 |
| Y | 2 | 0 | -1 |
| Z | -1 | 2 | 0 |

Supplementary Fig 10: **Evolutionary dynamics of RPS games under independent environmental noise on payoffs.** We assume that each element in the payoff matrix is subject to independent noise, and the intensity of noise of each element is proportional to the deterministic component of payoff matrix (with coefficient $k$, Eq. 80). For a negative-sum RPS (**a, b, c**), environmental noise can also induce a stable limit cycle (**b**), and can even make the interior equilibrium stable (**c**). For the other two cases (zero-sum RPS and positive-sum RPS), a noisy environment can strengthen the stability of the center and accelerate the convergence to the central equilibrium (**d-i**). All these scenarios show that environmental fluctuations – even multiple sources of noise – can strengthen the coexistence of different types, consistent with the reuslt in Fig. 4 in the main text. Parameters: $s = 0.1$.

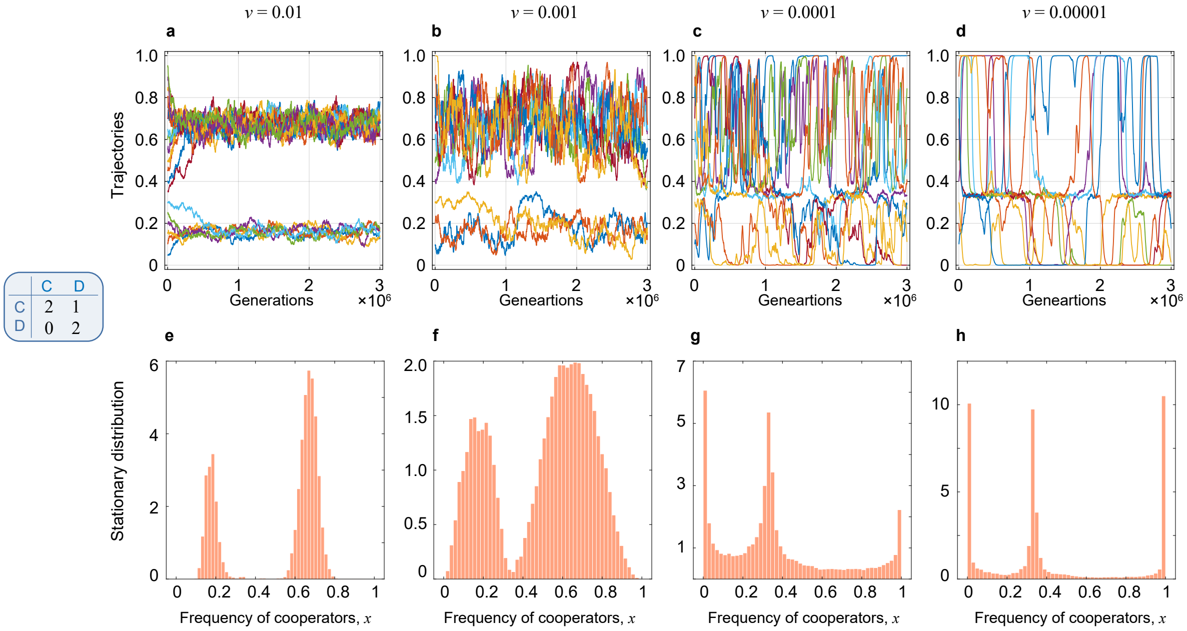


Supplementary Fig 11: **Evolutionary dynamics with colored environmental noise.** Colored noise means that the noise $\xi$ in generation $\tau+1$ is correlated with the noise in generation $\tau$, with correlation coefficient $1-\nu$ (Eq. 84). Thus, $\nu = 1$ corresponds to independent fluctuations in different generations (white noise), and $\nu = 0$ implies a constant environment without noise. We use a payoff structure with deterministic component $\bar{A} = [2,1;0,2]$ as an example to show the influence of colored noise. The evolutionary dynamics under white noise ($\nu = 1$) is shown by panel (**f**) in Fig. 2 in the main text. For a wide range of $\nu$ ($\nu \gg 1/N$), we find that the results are qualitatively consistent with the case of white noise (**a, b, e, f**). (**c, d, g, h**) When $\nu \sim 1/N$ or $\nu \ll 1/N$, the trajectories tend to stay near the stable equilibria (in noise-free case) of the payoff matrix $\bar{A}$ (with stable equilibria $x = 0$ and $x = 1$) and near $-\bar{A}$ (with stable equilibrium $x = 1/3$). Parameters: $s = 0.1$, $N = 20000$, $k = 2.5$.

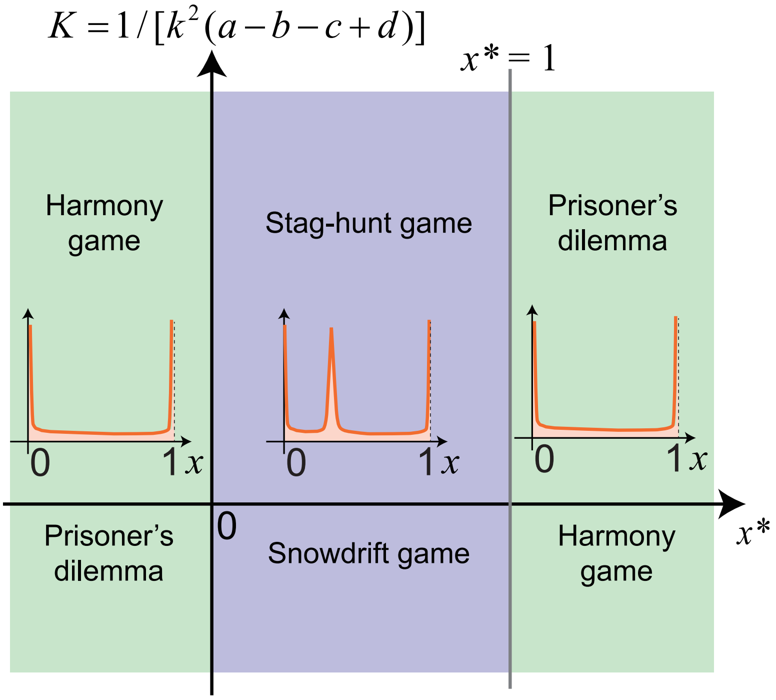


Supplementary Fig 12: **Stationary distributions in the limit of quenched noise.** In the limit of quenched noise ($\nu \to 0$), the environment fluctuates much more slowly than the evolution of strategy frequencies. Here we consider the case where the noise intensity is proportional to the mean payoff. In this regime, the stationary distributions of strategy frequencies for a harmony game or prisoner's dilemma have similar behavior: two humps near the boundary, at $x = 0$ and $x = 1$, which is different from the noise-free case. For a snowdrift game or a stag-hunt game, the stationary distributions are qualitatively different from the case without noise: two humps on the boundary ($x = 0$, $x = 1$) along with one hump in the interior $x = x^* = \frac{d-b}{a-b-c+d}$.

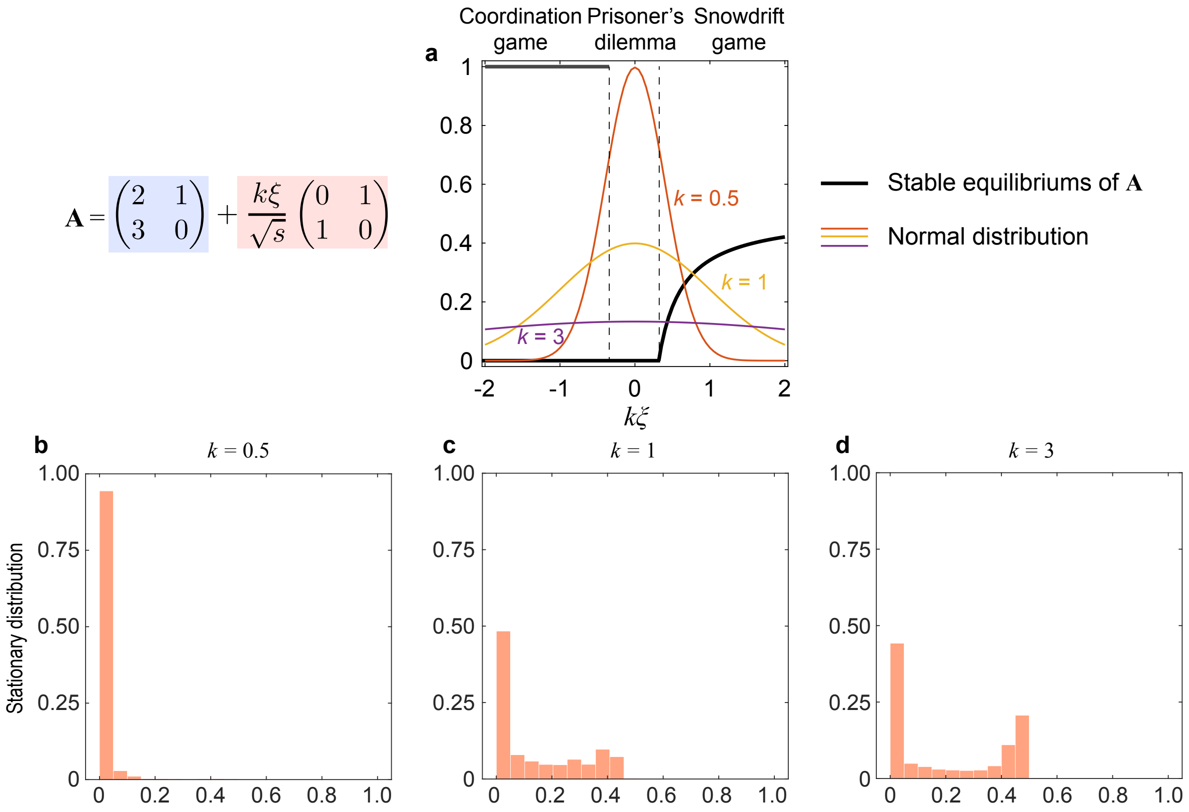


Supplementary Fig 13: **Stationary distributions for quenched noise not proportional to mean.** Here we consider an example where the noise intensity is not proportional to the mean payoff, in the regime $\nu \to 0$. We choose $\nu = 0.0001$, which can be seen as the quenched noise limit. Consider a prisoner's dilemma as an example. The noise intensity is controlled by a matrix $[0, k; k, 0]$. For different values of $k\xi$, the payoff matrix $A$ has different stable equilibria, which are shown by the black solid line in (a). Since the stationary distribution of $\xi$ is a standard normal distribution, the distributions of $k\xi$ for different values of $k$ are also illustrated. Given the relation between stable equilibria and the value of $\xi$, the stationary distribution of $x$ can also be computed by Eq. 91. We performed Monte Carlo simulations and plot the stationary distributions for different values of $k$. When $k$ is small, the distribution of $k\xi$ is most concentrated around 0, which corresponds to the classical equilibrium $x = 0$ (a). (b) When $k$ is larger, the non-zero stable equilibrium of $A$ has a higher probability. Thus the stationary distribution of $x$ also has substantial weight for $x \in [0, 0.5]$ (since as $\xi \to \infty$, the stable equilibrium of $A$ is $x = 0.5$) (c, d).

## Supplementary References


[1] Josef Hofbauer and Karl Sigmund. Evolutionary game dynamics. *Bull. Am. Math. Soc.*, 40(4):479–519, 2003.

[2] E. C. Zeeman. Population dynamics from game theory. In Zbigniew Nitecki and Clark Robinson, editors, *Global Theory of Dynamical Systems*, pages 471–497, Berlin, Heidelberg, 1980. Springer Berlin Heidelberg.

[3] John Guckenheimer and Philip Holmes. *Nonlinear oscillations, dynamical systems and bifurcations of vector fields*. Springer Science+Business Media, New York, 1983.

[4] Kenneth J. Arrow. *Essays in the Theory of Risk-Bearing*. Markham Economics Series. Markham Pub. Co, Chicago, 1971.

[5] John W Pratt. Risk Aversion in the Small and in the Large. In Peter Diamond and Michael Rothschild, editors, *Uncertainty in Economics*, pages 59–79. Academic Press, New York, 1978.

[6] Walter Nicholson and Christopher M. Snyder. *Microeconomic Theory: Basic Principles and Extensions*. Cengage Learning, 2012.

[7] Lasse Ruokolainen, Andreas Lindén, Veijo Kaitala, and Mike S. Fowler. Ecological and evolutionary dynamics under coloured environmental variation. *Trends Ecol. Evol.*, 24(10):555–563, 2009.

[8] Drew Fudenberg and Lorens A Imhof. Imitation processes with small mutations. *J. Econ. Theor.*, 131(1):251–262, 2006.

[9] Crispin W. Gardiner. *Handbook of stochastic methods: for physics, chemistry and the natural sciences*. Springer, Berlin Heidelberg, 2002.
